# Supplementary material for: Non-Markovian skin effect
Source: arXiv:2403.14455 source file (2024-09-23)
Supplement: Supplementary file 1 [file suppbib.tex]

\documentclass[pra,onecolumn,superscriptaddress,amssymb]{revtex4}
\usepackage[resetlabels]{multibib}
%\newcites{appendix}{Appendix literature}%  \cite, \nocitelatex, ...

\usepackage[colorlinks=true,linkcolor=magenta,citecolor=magenta,urlcolor=magenta,linktocpage=true]{hyperref}
%\pdfoutput=1
\usepackage{natbib}
\usepackage[utf8]{inputenc}
\usepackage[english]{babel}
\usepackage[T1]{fontenc}
\usepackage{amsmath}
\usepackage{cleveref}
\usepackage{svg}
\usepackage{tabularx}
\usepackage{array, makecell}

\usepackage{listings}
\usepackage{xcolor}
\makeatletter
\let\cat@comma@active\@empty
\makeatother

%------------------------------------------------------------------
\usepackage{listings}
\usepackage{xcolor}
\definecolor{codegreen}{rgb}{0,0.6,0}
\definecolor{codegray}{rgb}{0.5,0.5,0.5}
\definecolor{codepurple}{rgb}{0.58,0,0.82}
\definecolor{backcolour}{rgb}{0.95,0.95,0.92}
\lstdefinestyle{mystyle}{
    backgroundcolor=\color{backcolour},   
    commentstyle=\color{codegreen},
    keywordstyle=\color{magenta},
    numberstyle=\tiny\color{codegray},
    stringstyle=\color{codepurple},
    basicstyle=\ttfamily\footnotesize,
    breakatwhitespace=false,         
    breaklines=true,                 
    captionpos=b,                    
    keepspaces=true,                 
    numbers=none,                    
    numbersep=5pt,                  
    showspaces=false,                
    showstringspaces=false,
    showtabs=false,                  
    tabsize=2
}
\lstset{style=mystyle}
%\documentclass[twocolumn,showpacs,superscriptaddress,amssymb]{revtex4}

% Package(s) to include
\usepackage{psfrag,graphicx}
\usepackage{dcolumn}
\usepackage{bm}
\usepackage{amsfonts,amssymb,amsmath}        % for math symbols.
\usepackage{slashed}
\usepackage[utf8]{inputenc}\usepackage[caption=false]{subfig}
\usepackage{cancel}
\usepackage{xcolor}
\usepackage{amsmath}
\setcitestyle{numbers,square}

%\numberwithin{equation}{section}

%few extra commands from neill

%%%%%%%%%%%%%%%%%%%%%%%%%%%%%%%%%%
\newcommand{\be}{\begin{equation}}
\newcommand{\ee}{\end{equation}}
\newcommand{\bq}{\begin{eqnarray}}
\newcommand{\eq}{\end{eqnarray}}

\newcommand{\ket}[1]{\left |#1 \right\rangle}
\newcommand{\bra}[1]{\left \langle #1 \right |}

\newcommand{\bfj}{\textbf{j}}
\newcommand{\Symbol}[2]{{#1}_{\textrm{#2}}}

\newcommand{\s}{\text{s}}

\newcommand{\ADO}{\text{ADO}}

%%%%%%%%%%%%%%%%%%%%%%%%
\makeatletter

\renewenvironment{widetext@grid}{%
  \par\ignorespaces
  \setbox\widetext@top\vbox{%
   \vskip15\p@
   \hb@xt@\hsize{%
    \leaders\hrule\hfil
    \vrule\@height6\p@
   }%
   \vskip6\p@
  }%
  \setbox\widetext@bot\hb@xt@\hsize{%
    \vrule\@depth6\p@
    \leaders\hrule\hfil
  }%
  \onecolumngrid
%  \dimen@\ht\widetext@top\advance\dimen@\dp\widetext@top
%  \cleaders\box\widetext@top\vskip\dimen@
  \let\set@footnotewidth\set@footnotewidth@ii
}{%
  \par
%  \setbox\widetext@bot\vbox{%
%   \hb@xt@\hsize{\hfil\box\widetext@bot}%
%   \vskip14\p@
%  }%
%  \dimen@\ht\widetext@bot\advance\dimen@\dp\widetext@bot
%  \cleaders\box\widetext@bot\vskip\dimen@
  \twocolumngrid\global\@ignoretrue
  \@endpetrue
}%

%------------------------------------------------------------------
\begin{document}

\title{Supplemental Material: \\ Non-Markovian skin effect}
\author{Po-Chen Kuo}
% \author{Po-Chen Kuo\thanks{These authors contributed equally to this work. Email: pochen@phys.ncku.edu.tw}}
\email{These authors contributed equally to this work.}
\affiliation{Department of Physics, National Cheng Kung University, 701 Tainan, Taiwan}
\affiliation{Center for Quantum Frontiers of Research and Technology, NCKU, 701 Tainan, Taiwan}
\affiliation{Theoretical Quantum Physics Laboratory, Cluster for Pioneering Research, RIKEN, Wakoshi, Saitama 351-0198, Japan}
\author{Shen-Liang Yang}
% \author{Shen-Liang Yang\thanks{These authors contributed equally to this work}}
\email{These authors contributed equally to this work.}
\affiliation{Department of Physics, National Cheng Kung University, 701 Tainan, Taiwan}
\affiliation{Center for Quantum Frontiers of Research and Technology, NCKU, 701 Tainan, Taiwan}
\author{Neill Lambert}
\email{nwlambert@gmail.com}
\affiliation{Theoretical Quantum Physics Laboratory, Cluster for Pioneering Research, RIKEN, Wakoshi, Saitama 351-0198, Japan}
\author{Jhen-Dong Lin}
\affiliation{Department of Physics, National Cheng Kung University, 701 Tainan, Taiwan}
\affiliation{Center for Quantum Frontiers of Research and Technology, NCKU, 701 Tainan, Taiwan}
\author{Yi-Te Huang}
\affiliation{Department of Physics, National Cheng Kung University, 701 Tainan, Taiwan}
\affiliation{Center for Quantum Frontiers of Research and Technology, NCKU, 701 Tainan, Taiwan}
\author{Franco Nori}
\affiliation{Theoretical Quantum Physics Laboratory, Cluster for Pioneering Research, RIKEN, Wakoshi, Saitama 351-0198, Japan}
\affiliation{Center for Quantum Computing, RIKEN, Wakoshi, Saitama 351-0198, Japan}
\affiliation{Physics Department, The University of Michigan, Ann Arbor, Michigan 48109-1040, USA.}
\author{Yueh-Nan Chen}
\email{yuehnan@mail.ncku.edu.tw}
\affiliation{Department of Physics, National Cheng Kung University, 701 Tainan, Taiwan}
\affiliation{Center for Quantum Frontiers of Research and Technology, NCKU, 701 Tainan, Taiwan}

\setcounter{equation}{0}
\setcounter{figure}{0}
\renewcommand{\thefigure}{S\arabic{figure}}
\setcounter{section}{0}
\setcounter{table}{0}
\renewcommand{\thetable}{S\arabic{table}}
\setcounter{page}{1}
% \makeatletter
\maketitle
%\newrefsection
\appendix 
This supplemental material provides additional details, derivations, and supporting information related to the non-Markovian skin effect phenomena explored in the main text. It provides a deeper exploration of the theoretical framework, including the derivation of the Hierarchical equations of motion (HEOM) generator and its relation to the Born-Markov master equation (BMME) Liouvillian (Appendix A), decomposition of boson correlation functions (Appendix B), and diagonal decomposition of the HEOM Liouvillian superoperator (Appendix C). 

We explore the non-Markovian skin effect in a Lorentzian bath (Appendix D), examining memory effects and virtual processes in the strong coupling regime. The impact of collective and separated couplings to the bath is investigated (Appendix E), along with analyses of the scaled emission rate and inter-site coherence (Appendix F). 

Several appendices present key mathematical derivations, spectral decompositions of correlation functions, and detailed analyses of eigenvalue spectra and relaxation dynamics (Appendix G). Throughout, we provide comprehensive comparisons between Markovian and non-Markovian approaches under various conditions, offering insights into the unique characteristics of the non-Markovian skin effect.

\section{Derivation of the HEOM generator and its relation to the BMME Liouvillian}

Building upon the main text, we explore the HEOM generator and its use of auxiliary density operators (ADOs) within the ensemble ($\rho_{\text{s}+\text{ADO}}(t)$). We consider a generalized open quantum system (s) interacting with bosonic (b) environments described by the total (T) Hamiltonian ($\hbar=1$): 
\begin{equation}
\begin{aligned}
H_{\textrm{T}} = H_{\textrm{s}}(t) + H_{\textrm{b}} + H_{\textrm{sb}},
\label{eq:H_total}
\end{aligned}
\end{equation}
where $\Symbol{H}{s}(t)$ is the (possibly time-dependent) system Hamiltonian. The generic bosonic environment comprises multiple baths of non-interacting bosonic degrees of freedom:
\begin{equation}
\begin{aligned}
\Symbol{H}{b} = \sum_{\alpha}\sum_{k}\omega_{\alpha,k}a_{\alpha,k}^{\dagger}a_{\alpha,k},
\label{eq:H_b}
\end{aligned}
\end{equation}
where $a_{\alpha,k}$ $(a_{\alpha,k}^{\dagger})$ is the bosonic annihilation (creation) operator for the $k$th mode (frequency $\omega_{\alpha,k}$) in the $\alpha$th bosonic bath. This environment can represent various physical systems, e.g., electromagnetic environments~\cite{Mauro2016,Stockklauser2017}, phonons~\cite{Gustafsson2014,Iorsh2020}, surface plasmons~\cite{pochen2020}, or vibronic environments in molecules~\cite{Ishizaki_1_2009}.

The system-environment interaction is modeled by:
\begin{equation}
\begin{aligned}
\Symbol{H}{sb} = \Symbol{V}{s}\sum_{\alpha,k}g_{\alpha,k}(a_{\alpha,k}+a_{\alpha,k}^{\dagger})
\label{eq:H_sb}
\end{aligned}
\end{equation}
with coupling strengths $g_{\alpha,k}$. Here, $\Symbol{V}{s}$ are Hermitian coupling operators acting on the system's degrees of freedom, with even-parity for fermionic systems to ensure charge conservation. This model can be generalized to systems with multiple bosonic and fermionic quantum numbers interacting with individual or shared environments.

Applying the rotating wave approximation (RWA), we express $\Symbol{V}{s} = \Symbol{V}{s}^{+} + \Symbol{V}{s}^{-}$ in terms of raising ($+$) and lowering ($-$) operators. The interaction Hamiltonian is rewritten as:
\begin{equation}\label{H_RWA}
\begin{aligned}
\Symbol{H}{sb}^{\text{RWA}} = \sum_{\alpha,k}g_{\alpha,k}
(\Symbol{V}{s}^{+}a_{\alpha,k} + \Symbol{V}{s}^{-}a_{\alpha,k}^{\dagger}).
\end{aligned}
\end{equation}
To derive the HEOM, we assume: (1) The system and environments are initially separable, (2) Each bosonic bath is initially in thermal equilibrium, and (3) The bath operator in the system-bath interaction Hamiltonian is linear in bath annihilation and creation operators.

The reduced density matrix for the system at time $t$ is given by the Dyson series:
\begin{equation}\label{eq:G_series}
\begin{aligned}
\rho_{\textrm{s}}(t)=\hat{\mathcal{G}}(t)\left[\rho_{\textrm{s}}(0)\right],
\end{aligned}
\end{equation}
where the propagator $\hat{\mathcal{G}}(t)[\cdot]$ is a \textit{canonical superoperator}~\cite{Mauro2022}:
\begin{equation}
\begin{aligned}
\hat{\mathcal{G}}(t)[\cdot]
=\sum_{m=0}^{\infty}\frac{1}{m!}\hat{\mathcal{T}}\left\{-\int_{0}^{t} dt_1\int_{0}^{t_1}dt_2\left[\mathcal{W}_{\textrm{b}}(t_1,t_2)\right]\right\}^m
=\hat{\mathcal{T}}\exp\Big\{-\int_{0}^{t}d t_{1}\int_{0}^{t_{1}}d t_{2}
\hat{\mathcal{W}}_{\textrm{b}}(t_1,t_2)[\cdot]\Big\}
,\label{G_op}
\end{aligned}
\end{equation}
with the time-ordering operator $\hat{\mathcal{T}}$ and bosonic~\cite{Lambert2019,lambert2020bofinheom} operators:
\begin{equation}\label{W_op}
\begin{aligned}
\hat{\mathcal{W}}_{\textrm{b}}(t_1,t_2)[\cdot]
=\sum_{\alpha}\Big[\Symbol{V}{s}(t_1),
\left(
C^{\mathbb{R}}_{\alpha}(t_1,t_2)[\Symbol{V}{s}(t_2),\cdot]_{-}
+i C^{\mathbb{I}}_{\alpha}(t_1,t_2)[\Symbol{V}{s}(t_2),\cdot]_{+}
\right)\Big]_{-}.
\end{aligned}
\end{equation}
Here, $[\cdot,\cdot]_{-}$ and $[\cdot,\cdot]_{+}$ are commutator and anti-commutator, respectively. The bosonic environmental effects are encoded in the two-time correlation functions $C(t_1,t_2)$:
\begin{equation}
\begin{aligned}
C_{\alpha}(t_{1},t_{2})
=\frac{1}{2\pi}\int_{0}^{\infty} d\omega 
J_{\alpha}(\omega)\Big[n_{\alpha}^{\textrm{eq}}(\omega)e^{i\omega (t_{1}-t_{2})}
+(n_{\alpha}^{\textrm{eq}}(\omega)+1)e^{-i\omega (t_{1}-t_{2})}
\Big],
\label{eq:C_b}
\end{aligned}
\end{equation}
where $J_{\alpha}(\omega)=2\pi\sum_{k} g_{\alpha,k}^{2}\delta(\omega-\omega_{k})$ is the spectral density and $n_{\alpha}^{\textrm{eq}}(\omega)=\{\exp[\omega/k_{\textrm{B}}T_{\alpha}]-1\}^{-1}$ is the Bose–Einstein distribution.

A practical representation of Eq.~(\ref{eq:G_series}) expresses bath correlation functions as a sum of exponentials:
\begin{equation}
\begin{aligned}
C_{\alpha}(\tau)=\sum_{l=1}^{l_{\text{max},\alpha}}\xi_{\alpha,l}\exp(-\chi_{\alpha,l}\tau), 
\label{eq:C_b_exp}
\end{aligned}
\end{equation}
where $\tau=t_{1}-t_{2}$, and $l_{\text{max},\alpha}$ is the total number of exponentials for the $\alpha$-bosonic bath. When $\chi_{\alpha,l}\neq\chi_{\alpha,l}^*$, we decompose the bosonic correlation function into real ($\mathbb{R}$) and imaginary ($\mathbb{I}$) parts:
\begin{equation}
\begin{aligned}
C_{\alpha}(\tau) = \sum_{u=\mathbb{R},\mathbb{I}} 
(\delta_{u,\mathbb{R}}+i\delta_{u,\mathbb{I}})C_{\alpha}^{u}(\tau),
\label{eq:C_beta_RI}
\end{aligned}
\end{equation}
where
\begin{equation}
\begin{aligned}
C_{\alpha}^{u}(\tau) = \sum_{l=1}^{l_{max,\alpha}^u}
\xi_{\alpha,l}^{u}\exp(-\chi_{\alpha,l}^{u}\tau).
\label{eq:C_beta_u}
\end{aligned}
\end{equation}

Using these expressions in Eq.~(\ref{G_op}) and recursive differentiation in time~\cite{Mauro2022,KondoQED2023}, we define a local master equation in an enlarged space of \textit{auxiliary density operators} (ADOs) $\rho^{(m)}_{\bfj}(t)$. These ADOs encode the environment's influence~\cite{Tanimura07}, each linked to an exponential term in the correlation function decomposition. The HEOM generator can be expressed as~\cite{Mauro2022,Huang2023}:
\begin{equation}
\begin{aligned}
\mathcal{L}_{\text{H}}[\rho^{(m)}_{\bfj}(t)]
=\mathcal{L}_{0}[\rho^{(m)}_{\bfj}(t)]
-\sum_{r=1}^{m}\chi_{j_{r}}\rho^{(m)}_{\bfj}(t)
-i\sum_{j'} \mathcal{A}_{j'}
[\rho^{(m+1)}_{\bfj^+}(t)]
-i\sum_{r=1}^{m}\mathcal{B}_{j_{r}}
[\rho^{(m-1)}_{\bfj_{r}^{-}}(t)],
\label{eq:HEOML}
\end{aligned}
\end{equation}
where $\bfj=[j_m,\cdots,j_1]$, $\bfj^{+}=[j',j_{m},\cdots,j_1]$, and $\bfj_{r}^{-}=[j_m,\cdots,j_{r+1},j_{r-1},\cdots,j_{1}]$. Each $j$ corresponds to a multi-index ensemble $\{\alpha,u,l\}$, where the multi-index $\alpha$ represents different baths, $u$ denotes real ($\mathbb{R}$) or imaginary ($\mathbb{R}$) parts of the correlation function, and $l$ indexes the exponential terms in the correlation function decomposition.

The system-bath interactions are encoded through superoperators $\hat{\mathcal{A}}_{j}$, $\hat{\mathcal{B}}_{j}$:
\begin{equation}
\begin{aligned}
&\mathcal{L}_{0}[\cdot]=-i[H_{\text{s}},\cdot]_{-}\\
&\mathcal{A}_{j}[\cdot] = [\Symbol{V}{s},\cdot]_{-}\\
&\mathcal{B}_{j}[\cdot] = \delta_{u,\mathbb{R}}\xi^{\mathbb{R}}_{n,l}[\Symbol{V}{s},\cdot]_{-}+i\delta_{u,\mathbb{I}}\xi^{\mathbb{I}}_{n,l}[\Symbol{V}{s},\cdot]_{+}.
\end{aligned}
\end{equation}

\subsection{RWA-HEOM: Implementing the rotating-wave approximation in HEOM}
Under the RWA, the superoperator in Eq.~(\ref{W_op}) simplifies to
\begin{equation}\label{W_RWA}
\begin{aligned}
\hat{\mathcal{W}}_{\textrm{b}}^{\text{RWA}}(t_1,t_2)[\cdot]
= \sum_{\alpha}\sum_{\nu=\pm}\Big[\Symbol{V}{s}^{\bar{\nu}}(t_1), \left(C^{\nu}_{\alpha}(t_1 - t_2) \Symbol{V}{s}^{\nu}(t_2)[\cdot] + C^{\bar{\nu}\ast}_{\alpha}(t_1 - t_2) [\cdot] \Symbol{V}{s}^{\nu}(t_2)\right)\Big]_{-},
\end{aligned}
\end{equation}
where the correlation function separates into absorption $(\nu = +)$ and emission $(\nu =-)$ components:
\begin{equation}\label{C_RWA}
    \begin{aligned}
        &C^{+}_{\alpha}(t)
        =\frac{1}{2\pi}\int_{0}^{\infty} d\omega 
        J_{\alpha}(\omega)n^{\textrm{eq}}_{\alpha}(\omega)e^{i\omega \tau}
        =\sum_{l}^{l_{\text{max}}}\xi_{\alpha,l}^{\nu=+}\exp(-\chi_{l}^{\nu=+}\tau),\\
        &C^{-}_{\alpha}(t)=\frac{1}{2\pi}\int_{0}^{\infty} d\omega 
J_{\alpha}(\omega)[n^{\textrm{eq}}_{\alpha}(\omega)+1]e^{-i\omega \tau}
=\sum_{l}^{l_{\text{max}}}\xi_{l}^{\nu=-}\exp(-\chi_{l}^{\nu=-}\tau).
    \end{aligned}
\end{equation}
Specifically, if $\nu = +$, then $\bar{\nu} = -$, and vice versa.
The corresponding extended Liouvillian superoperator under RWA is:
\begin{equation}\label{eq:HEOML_RWA}
    \begin{aligned}
        \mathcal{L}_{\text{s}+\text{ADO}}^{\text{RWA}}[\rho^{(m)}_{\bfj}(t)]
        =\mathcal{L}_{0}[\rho^{(m)}_{\bfj}(t)]
        -\sum_{r=1}^{m}\chi_{j_{r}}\rho^{(m)}_{\bfj}(t)
        -i\sum_{j'} \mathcal{A}_{j'}
        [\rho^{(m+1)}_{\bfj^+}(t)]
        -i\sum_{r=1}^{m}\mathcal{B}_{j_{r}}(0)
        [\rho^{(m-1)}_{\bfj_{r}^{-}}(t)],
        \end{aligned}
    \end{equation}
with the modified superoperators:
\begin{equation}\label{mod_sup_AC}
\begin{aligned}
\mathcal{A}_{j}[\cdot] = [\Symbol{V}{s}^{\bar{\nu}},\cdot]_{-}~~~\text{and}~~~
\mathcal{B}_{j}(t)[\cdot] = C^{\nu}_{\alpha}(t) \Symbol{V}{s}^{\nu}[\cdot] + C^{\bar{\nu}\ast}_{\alpha}(t) [\cdot] \Symbol{V}{s}^{\nu}.
\end{aligned}
\end{equation}
However, when $t=0$, $\mathcal{B}_{j}(0)[\cdot]$ simplifies as follows
\begin{equation}
\begin{aligned}
\mathcal{B}_{j}(0)[\cdot] = \xi^{\nu}_{l}~\Symbol{V}{s}^{\nu}[\cdot]-\xi^{\bar{\nu}\ast}_{l}[\cdot]~\Symbol{V}{s}^{\nu}.
\end{aligned}
\end{equation}

\subsection{BMME: Implementing the Born-Markov approximation in RWA-HEOM}

The Born approximation, which typically involves neglecting higher-order terms in the influence functional, is not required in this context. Due to the Gaussian nature of the bath and our utilization of Wick's theorem for superoperators, all the higher-order terms in Eq.~(\ref{eq:G_series}) [i.e., $m > 2$ in Eq.~(\ref{eq:G_series})] can be expressed as products of the second-order terms.

Substituting Eq.~(\ref{W_RWA}) into Eq.~(\ref{eq:G_series}) and taking the time derivative yield the exact master equation:
\begin{equation}\label{nMME}
\begin{aligned}
\partial_t \rho_{\text{s}}(t)= -\frac{i}{\hbar}[H_\text{s}(t),\rho_{\text{s}}(t)]
-\hat{\mathcal{T}}\sum_{j = \alpha,\nu}
\mathcal{A}_{j}\left[\int_0^t dt_{1} \mathcal{B}_{j}(t-t_1)[\rho(t)]\right].
\end{aligned}
\end{equation}
This equation is time-nonlocal due to the presence of the memory kernel (responsibles for the memory effect), $\int_0^t dt_1 \mathcal{B}_{j}(t-t_1)$, which embodies the influence of the bosonic bath on the system's dynamics. 

The Markov approximation posits that the system's dynamics are memoryless, implying that its future evolution depends solely on its present state. This assumption holds when the bath correlation time is significantly shorter than the system's characteristic timescale, as reflected in the reduced system density matrix $\rho_{\text{s}}$. This short correlation time signifies the rapid ``forgetting'' of past system-bath interactions, leading to Markovian behavior. Consequently, for sufficiently large $(t-t_1)$ in Eq.~(\ref{nMME}), the oscillating exponential averages the slowly varying functions $J_{\alpha}(\omega)$ and $n^{\text{eq}}_{\alpha}(\omega)$ to zero.
Mathematically, the absence of memory effects is manifested when the two-time correlation functions are proportional to the Dirac delta function, namely:
\begin{equation}\label{delta_Corr}
\begin{aligned}
C_{\alpha}^{\nu}(t, t_1) \propto \delta(t - t_1).
\end{aligned}
\end{equation}
A sufficient condition for the Markovian regime (resonance regime) is that both the spectral density $J(\omega) = J(\Omega)$ and the Bose-Einstein distribution $n(\omega) = n(\Omega)$ resonate with the system's transition frequency $\Omega$, becoming frequency-independent constants. This resonance facilitates rapid energy exchange between the system and bath, effectively erasing the memory effects.
Thus, we can evaluate the two-time correlation functions for the bosonic baths in Eq.~(\ref{C_RWA}):
\begin{equation}
C_{\alpha}^{\nu}(t,t_1) = \frac{1}{2\pi} \int_{0}^{\infty} d\omega J_{\alpha}(\Omega) [\delta_{\nu,-1} + n_{\alpha}^{\text{eq}}(\Omega)] e^{\nu i \omega (t - t_1)} 
= J_{\alpha}(\Omega) [\delta_{\nu,-1} + n_{\alpha}^{\text{eq}}(\Omega)] \delta(t - t_1),
\end{equation}
where $\delta_{\nu,\nu'}$ is the Kronecker delta, equal to unity when $\nu=\nu'$ and zero otherwise.

By substituting the above Markovian approximation of the correlation function into Eq.~(\ref{mod_sup_AC}) and then applying it to Eq.~(\ref{nMME}), the memory kernel term in the exact master equation becomes
\begin{equation}\label{memory_ker}
\begin{aligned}
\hat{\mathcal{T}}\sum_{\nu = \pm 1} \mathcal{A}_{j}&\left[\int_0^t dt_{1} \mathcal{B}_{j}(t-t_1)[\cdot]\right]
= \sum_{\nu = \pm 1} \mathcal{A}_{j}\left[ \left( \int_0^t dt_1 C_\alpha^\nu(t, t_1) \right) V_{\text{s}}^\nu [\cdot] - \left( \int_0^t dt_1 C_\alpha^{\bar{\nu}\ast}(t, t_1) \right) [\cdot] V_{\text{s}}^\nu \right]\\
&= \frac{1}{2} J_\alpha(\Omega) \sum_{\nu = \pm 1} \mathcal{A}_{j} \left[ \left( \delta_{\nu, -1} + n_\alpha^{\text{eq}}(\Omega) \right) V_{\text{s}}^\nu [\cdot] - \left( \delta_{\bar{\nu}, -1} + n_\alpha^{\text{eq}}(\Omega) \right) [\cdot] V_{\text{s}}^\nu \right]\\
&= \frac{1}{2} J_\alpha(\Omega) \Big\{n_\alpha^{\text{eq}}(\Omega) \left[ V_{\text{s}}^{-} V_{\text{s}}^{+} [\cdot] - V_{\text{s}}^{+} [\cdot] V_{\text{s}}^{-} \right] + \left( 1 + n_\alpha^{\text{eq}}(\Omega) \right) \left[ [\cdot] V_{\text{s}}^{+}V_{\text{s}}^{-} - V_{\text{s}}^{-} [\cdot] V_{\text{s}}^{+} \right]\\
&+n_\alpha^{\text{eq}}(\Omega) \left[ [\cdot]V_{\text{s}}^{-} V_{\text{s}}^{+}  - V_{\text{s}}^{+} [\cdot] V_{\text{s}}^{-} \right] + \left( 1 + n_\alpha^{\text{eq}}(\Omega) \right) \left[ V_{\text{s}}^{+}V_{\text{s}}^{-}[\cdot]  - V_{\text{s}}^{-} [\cdot] V_{\text{s}}^{+} \right]\Big\}\\
&= \frac{1}{2} J_\alpha(\Omega) \Big\{ n_\alpha^{\text{eq}}(\Omega) \left( \left[V_{\text{s}}^{-} V_{\text{s}}^{+},\cdot\right]_{+} - 2V_{\text{s}}^{+} [\cdot] V_{\text{s}}^{-} \right) + \left( 1 + n_\alpha^{\text{eq}}(\Omega) \right) \left( \left[V_{\text{s}}^{+} V_{\text{s}}^{-},\cdot\right]_{+}  - 2V_{\text{s}}^{-} [\cdot] V_{\text{s}}^{+} \right) \Big\}.
\end{aligned}
\end{equation}

Upon substituting Eq.~(\ref{memory_ker}) back into Eq.~(\ref{nMME}), we obtain the Born-Markov master equation (BMME)
\begin{equation}
\begin{aligned}
\partial_{t} \rho_{\text{s}}(t) = -i[\hat{H}_{\text{s}},\rho_{\text{s}}(t)] 
+ \sum_{\alpha} \left\{ \mathcal{J}_{\alpha}(L_{\text{abs}})[\rho_{\text{s}}(t)] + \mathcal{J}_{\alpha}(L_{\text{emi}})[\rho_{\text{s}}(t)]\right\},
\end{aligned}
\end{equation}
where the Lindblad operators $L_{\text{emi}}$ and $L_{\text{abs}}$ characterize the emission and absorption processes, respectively, induced by the system-bath interaction
\begin{equation}
\begin{aligned}
L_{\text{emi}}=\sqrt{J_{\alpha}(\Omega)\left[n_{\alpha}^{\text{eq}}(\Omega)+1\right]}V_{\text{s}},
\end{aligned}
\end{equation}
\begin{equation}
\begin{aligned}
L_{\text{abs}}=\sqrt{J_{\alpha}(\Omega)n_{\alpha}^{\text{eq}}(\Omega)}V_{\text{s}}^{\dagger}.
\end{aligned}
\end{equation}
Here, $\mathcal{J}_{\alpha}(L)$ is the bosonic Lindbladian dissipator, which describes the dissipative interaction between the system and the environment for a given Lindblad operator $L$. Its explicit form is given by
\begin{equation}
\begin{aligned}
\mathcal{J}_{\alpha}(L)[\cdot] &= L[\cdot]L^\dagger - \frac{1}{2}\{L^\dagger L, \cdot \}_+.
\end{aligned}
\end{equation} 

\section{Decomposition of Boson correlation functions}\label{sec1}

\subsection{Pad\'{e} decomposition for the Drude-Lorentz spectral density}
This section presents an example of decomposing an $\alpha$-bosonic reservoir correlation function into a sum of $l_{\text{max},\alpha}$-exponential terms. We focus specifically on the following Drude-Lorentz spectral density:
\begin{equation}\label{eq:Drude-Lorentz}
     J_\alpha(\omega)=\frac{4\Gamma_\alpha W_\alpha\omega}{\omega^2+W_\alpha^2},
\end{equation}
where $\Gamma_\alpha$ represents the system-reservoir coupling strength for the $\alpha$-bosonic reservoir with bandwidth $W_\alpha$. We express the Bose-Einstein distribution $n_{\alpha}^{\textrm{eq}}(x)=\{\exp(x)-1\}^{-1}$ as a series via the Pad\'{e} decomposition~\cite{Jie2011}:
\begin{equation}
    n_{\alpha}^{\textrm{eq}}(x)\approx n_{\alpha}^\textrm{Pad\'{e}}(x)=\frac{1}{x}-\frac{1}{2}+\sum_{l=2}^{l_{\text{max},\alpha}}\frac{2\kappa_l x}{x^2+\zeta_l^2}.
\end{equation}
Here, $\kappa_l$ and $\zeta_l$ are parameters described in~\cite{Jie2011} and depend on  $l_{\text{max},\alpha}$. Employing this decomposition and the residue theorem, we can analytically evaluate the integration from Eq.~(4) of the main text:
\begin{equation}
    C_\alpha(\tau)\approx\sum_{l=1}^{l_{\text{max},\alpha}}\xi_{\alpha,l}\exp(-\chi_{\alpha,l} \tau)
\end{equation}
with
\begin{equation}
\begin{aligned}
    \xi_{\alpha,1} &= \Gamma_\alpha W_\alpha \left[-i+\cot\left(\frac{W_\alpha}{2 k_{\textrm{B}} T}\right)\right],\\
    \chi_{\alpha,1} &=W_\alpha,\\
    \xi_{\alpha,l\neq1} &= -2 \kappa_l k_{\textrm{B}} T \cdot \frac{2 \Gamma_\alpha W_\alpha \cdot \zeta_l k_{\textrm{B}} T}{-(\zeta_l k_{\textrm{B}} T)^2 + W_\alpha^2},\\
    \chi_{\alpha,l\neq1} &= \zeta_l k_{\textrm{B}} T.\\
\end{aligned}
\end{equation}
Notably, the bosonic correlation function in this case does not require further separation into real and imaginary parts due to the property $\chi_{\alpha, l}=\chi_{\alpha, l}^* ~\forall~ l$.

\subsection{Adaptive Antoulas-Anderson algorithm barycentric spectrum decomposition for the Drude-Lorentz spectral density with rotating-wave approximation}

We employ the adaptive Antoulas-Anderson (tA) algorithm, based on the barycentric representation \cite{Meng2022, AAA-algorithm}, to numerically identify the minimal sum-of-pole structure for the bosonic reservoir spectrum characterized by a Drude-Lorentz spectral density [Eq.~(\ref{eq:Drude-Lorentz})] under the rotating wave approximation (RWA).
Given a general real function $f(\omega)$, its sum-of-pole expansion can be obtained using high-precision rational approximations on the real axis. This is achieved by expressing the function under a barycentric representation $f^{\textrm{tA}}$:
\begin{align}
f(\omega)\approx f^{\textrm{tA}}(\omega)=\sum_{j=1}^{m}\sum_{\nu=+,-}\frac{R_f(\omega_j^\nu)}{\omega-\omega_j^\nu},
\end{align}
where $\omega_j^+$ ($\omega_j^-$) are the poles of $f^{\textrm{tA}}$ in the upper (lower) half-plane, and $R_f$ gives the corresponding residues. As $f$ is real, poles appear in conjugate pairs: $\omega_j^- = (\omega_j^+)^*~\forall~j$. Once $\omega_j^\nu$ and $R_f(\omega_j^\nu)$ are numerically determined by the AAA algorithm, we compute the Fourier transform of $f^\textrm{tA}(\omega)$ for $t\geq0$:
\begin{align}
\int_{-\infty}^{\infty} f^\textrm{tA}(\omega) e^{i \omega t}d\omega &= \sum_{j=1}^m \sum_\nu \int_{-\infty}^{\infty} \frac{R_f(\omega_j^\nu) e^{i \omega t}}{\omega-\omega_j^\nu} d\omega = \sum_{j=1}^m 2\pi i R_f(\omega_j^+) e^{i\omega_j^+ t},\label{eq:aaa-fourier-plus}\\
\int_{-\infty}^{\infty} f^\textrm{tA}(\omega) e^{-i \omega t}d\omega &= \sum_{j=1}^m \sum_\nu \int_{-\infty}^{\infty} \frac{R_f(\omega_j^\nu) e^{-i \omega t}}{\omega-\omega_j^\nu} d\omega = \sum_{j=1}^m -2\pi i R_f(\omega_j^-) e^{-i\omega_j^- t}.\label{eq:aaa-fourier-minus}
\end{align}
The second equality in both equations follows from the residue theorem and Jordan's lemma. These equations are useful for decomposing the Bose-Einstein distribution and arbitrary spectral density of a bosonic reservoir.
To apply this to our case, we first divide the absorption and emission components of the correlation function [Eq.~(\ref{C_RWA})] into real and imaginary parts:
\begin{align}
C^{+}_{\alpha}(t) &= C^{+\mathbb{R}}_{\alpha}(t)+iC^{+\mathbb{I}}_{\alpha}(t) = \frac{1}{2\pi}\int_{0}^{\infty} d\omega J_{\alpha}(\omega)n^{\textrm{eq}}_{\alpha}(\omega)\text{cos}(\omega t)+\frac{i}{2\pi}\int_{0}^{\infty} d\omega J_{\alpha}(\omega)n^{\textrm{eq}}_{\alpha}(\omega)\text{sin}(\omega t),\label{c_RWA_abs}\\
C^{-}_{\alpha}(t) &= C^{-\mathbb{R}}_{\alpha}(t)+iC^{-\mathbb{I}}_{\alpha}(t) = \frac{1}{2\pi}\int_{0}^{\infty} d\omega J_{\alpha}(\omega)[n^{\textrm{eq}}_{\alpha}(\omega)+1]\text{cos}(\omega t)-\frac{i}{2\pi}\int_{0}^{\infty} d\omega J_{\alpha}(\omega)[n^{\textrm{eq}}_{\alpha}(\omega)+1]\text{sin}(\omega t).\label{c_RWA_emi}
\end{align}
For contour integration, $J_{\alpha}(\omega)$ must be even in its real part and odd in its imaginary part, and $n^{\textrm{eq}}_{\alpha}(\omega)$ must be even. We then rewrite the equations as:
\begin{align}
C^{+\mathbb{R}}_{\alpha}(t) &= \frac{1}{8\pi}\int_{-\infty}^{\infty} d\omega J_{\alpha}^{\textrm{(even)}}(\omega)n^{\textrm{eq(even)}}_{\alpha}(\omega)[e^{i\omega t}+e^{-i\omega t}],\label{c_RWA_abs_R}\\
C^{+\mathbb{I}}_{\alpha}(t) &= \frac{1}{8\pi}\int_{-\infty}^{\infty} d\omega J_{\alpha}^{\textrm{(odd)}}(\omega)n^{\textrm{eq(even)}}_{\alpha}(\omega)[e^{i\omega t}-e^{-i\omega t}],\label{c_RWA_abs_I}\\
C^{-\mathbb{R}}_{\alpha}(t) &= \frac{1}{8\pi}\int_{-\infty}^{\infty} d\omega J^{\textrm{(even)}}_{\alpha}(\omega)[n^{\textrm{eq(even)}}_{\alpha}(\omega)+1][e^{i\omega t}+e^{-i\omega t}],\label{c_RWA_emi_R}\\
C^{-\mathbb{I}}_{\alpha}(t) &= \frac{-1}{8\pi}\int_{-\infty}^{\infty} d\omega J^{\text{(odd)}}_{\alpha}(\omega)[n^{\textrm{eq(even)}}_{\alpha}(\omega)+1][e^{i\omega t}-e^{-i\omega t}],\label{c_RWA_emi_I}
\end{align}
where
\begin{align}\label{even_odd_f}
J^{\text{(odd)}}_{\alpha}(\omega) &= \begin{cases}
J_{\alpha}(\omega), &\omega\geq 0\\
-J_{\alpha}(-\omega), &\omega< 0
\end{cases},\\
J^{\text{(even)}}_{\alpha}(\omega) &= \begin{cases}
J_{\alpha}(\omega), &\omega\geq 0\\
J_{\alpha}(-\omega), &\omega< 0
\end{cases},\\
n^{\textrm{eq(even)}}_{\alpha}(\omega) &= \begin{cases}
n^{\textrm{eq}}_{\alpha}(\omega), &\omega\geq 0\\
n^{\textrm{eq}}_{\alpha}(-\omega), &\omega< 0
\end{cases}.
\end{align}
We then numerically find the pole structure of $J^{\text{(odd)}}_{\alpha}, J^{\text{(even)}}_{\alpha},$ and $n^{\textrm{eq(even)}}_{\alpha}$ using the AAA algorithm:
\begin{equation}
\begin{aligned}
J^{\text{(odd)}}_{\alpha}(\omega) &\approx \tilde J^{\text{(odd)}}_{\alpha}(\omega)=\sum_{i=1}^{l}\sum_{\nu=+,-}\frac{R_{J_{\text{odd}}}(\omega_i^\nu)}{\omega-\omega_i^\nu},\\
J^{\text{(even)}}_{\alpha}(\omega) &\approx \tilde J^{\text{(even)}}_{\alpha}(\omega)=\sum_{j=1}^{m}\sum_{\nu=+,-}\frac{R_{J_{\text{even}}}(\omega_j^\nu)}{\omega-\omega_j^\nu},\\
n^{\textrm{eq(even)}}_{\alpha}(\omega) &\approx \tilde n^{\textrm{eq(even)}}_{\alpha}(\omega)=\sum_{k=1}^{n}\sum_{\nu=+,-}\frac{R_{n_{\text{even}}}(\omega_k^\nu)}{\omega-\omega_k^\nu}.\label{residues}
\end{aligned}
\end{equation}
Substituting Eq.~(\ref{residues}) into Eqs.~(\ref{c_RWA_abs_R})-(\ref{c_RWA_emi_I}) and solving the contour integral by the residue theorem:
\begin{equation}
\begin{aligned}
C^{+}_{\alpha}(t) &= \frac{i}{4}\sum^m_{j=1} R_{J_{\text{even}}}(\omega_j^+) \tilde n^{\textrm{eq(even)}}_{\alpha}(\omega_j^+)e^{-(-i\omega_j^+)t}-\frac{i}{4}\sum^m_{j=1} R_{J_{\text{even}}}(\omega_j^-) \tilde n^{\textrm{eq(even)}}_{\alpha}(\omega_j^-)e^{-(i\omega_j^-)t}\\
&+\frac{i}{4}\sum^l_{i=1} R_{J_{\text{odd}}}(\omega_i^+) \tilde n^{\textrm{eq(even)}}_{\alpha}(\omega_i^+)e^{-(-i\omega_i^+)t}+\frac{i}{4}\sum^l_{i=1} R_{J_{\text{odd}}}(\omega_i^-) \tilde n^{\textrm{eq(even)}}_{\alpha}(\omega_i^-)e^{-(i\omega_i^-)t}\\
&+\frac{i}{4}\sum^n_{k=1} [\tilde J^{\text{(odd)}}_{\alpha}(\omega_k^+)+\tilde J^{\text{(even)}}_{\alpha}(\omega_k^+)] R_{n_{\text{even}}}(\omega_k^+) e^{-(-i\omega_k^+)t}\\
&+\frac{i}{4}\sum^n_{k=1} [\tilde J^{\text{(odd)}}_{\alpha}(\omega_k^-)-\tilde J^{\text{(even)}}_{\alpha}(\omega_k^-)] R_{n_{\text{even}}}(\omega_k^-) e^{-(i\omega_k^-)t},\label{c_RWA_abs_final}
\end{aligned}
\end{equation}
and
\begin{equation}
\begin{aligned}
C^{-}_{\alpha}(t) &= \frac{i}{4}\sum^m_{j=1} R_{J_{\text{even}}}(\omega_j^+) [\tilde n^{\textrm{eq(even)}}_{\alpha}(\omega_j^+)+1]e^{-(-i\omega_j^+)t}-\frac{i}{4}\sum^m_{j=1} R_{J_{\text{even}}}(\omega_j^-) [\tilde n^{\textrm{eq(even)}}_{\alpha}(\omega_j^-)+1]e^{-(i\omega_j^-)t}\\
&-\frac{i}{4}\sum^l_{i=1} R_{J_{\text{odd}}}(\omega_i^+) [\tilde n^{\textrm{eq(even)}}_{\alpha}(\omega_i^+)+1]e^{-(-i\omega_i^+)t}-\frac{i}{4}\sum^l_{i=1} R_{J_{\text{odd}}}(\omega_i^-) [\tilde n^{\textrm{eq(even)}}_{\alpha}(\omega_i^-)+1]e^{-(i\omega_i^-)t}\\
&+\frac{i}{4}\sum^n_{k=1} [\tilde J^{\text{(odd)}}_{\alpha}(\omega_k^+)-\tilde J^{\text{(even)}}_{\alpha}(\omega_k^+)] R_{n_{\text{even}}}(\omega_k^+) e^{-(-i\omega_k^+)t}\\
&-\frac{i}{4}\sum^n_{k=1} [\tilde J^{\text{(odd)}}_{\alpha}(\omega_k^-)+\tilde J^{\text{(even)}}_{\alpha}(\omega_k^-)] R_{n_{\text{even}}}(\omega_k^-) e^{-(i\omega_k^-)t}.\label{c_RWA_emi_final}
\end{aligned}
\end{equation}
We combine the real and imaginary parts in absorption and emission components, and merge exponents from real and imaginary parts into a single exponent if they are equal~\cite{lambert2020bofinheom}. This decomposition of absorption and emission components into the sum of exponential terms can be substituted into the HEOM [Eq.~(\ref{eq:HEOML_RWA})]. A numerical analysis of this procedure yields 2 poles for $J_{\text{odd}}(\omega)$, 9 poles for $J_{\text{even}}(\omega)$, and 6 poles for $n(\omega)$, resulting in a total of 32 terms in the exponential expansion.

\subsection{Spectrum decomposition for Lorentzian spectral density at zero temperature}

In our alternative abstract model, we consider a bosonic bath with a Lorentzian spectral density:
\begin{equation}
J_{\alpha}(\omega) = \frac{1}{2\pi} \frac{\Gamma W^2}{(\omega - \omega_0)^2 + W^2}.
\end{equation}
For simplicity, we consider absolute zero temperature and that the dominant bath frequency is far from zero. Consequently, Eq.~(\ref{eq:C_b}) is simplified as:
\begin{equation}
C_{\alpha}(t_{1},t_{2}) \approx\frac{1}{2\pi}\int_{-\infty}^{\infty} d\omega J_{\alpha}(\omega)e^{-i\omega (t_{1}-t_{2})}. \label{C_b_L}
\end{equation}
Using complex integration and the residue theorem, this correlation can be decomposed in the form of Eq.~(\ref{eq:C_beta_RI}):
\begin{equation}\label{eq:C_Lor_RI}
C_{\alpha}(\tau) = C_{\alpha}^{\mathbb{R}}(\tau)+iC_{\alpha}^{\mathbb{I}}(\tau)=\sum_{l=1}^{2} \left[\xi_{\alpha,l}^{\mathbb{R}}\exp(-\chi_{\alpha,l}^{\mathbb{R}}(\tau) +i\xi_{\alpha,l}^{\mathbb{I}}\exp(-\chi_{\alpha,l}^{\mathbb{I}}(\tau)\right],
\end{equation}
where
\begin{equation}\label{eq:coeff_Lor_RI}
\begin{aligned}
&\xi_{\alpha,1}^{\mathbb{R}} = \xi_{\alpha,2}^{\mathbb{R}} = \frac{\Gamma W}{4},~~ 
\chi_{\alpha,1}^{\mathbb{R}} = W+i\omega_{0},~~\chi_{\alpha,2}^{\mathbb{R}} = W-i\omega_{0}\\
&\xi_{\alpha,1}^{\mathbb{I}} = -i\frac{\Gamma W}{4}, ~~\xi_{\alpha,2}^{\mathbb{I}} = i\frac{\Gamma W}{4},~~ 
\chi_{\alpha,1}^{\mathbb{I}} = W+i\omega_{0},~~\chi_{\alpha,2}^{\mathbb{I}} = W-i\omega_{0}.
\end{aligned}
\end{equation}
These coefficients can be substituted into Eq.~(\ref{eq:HEOML}) to obtain the HEOM generator. 
Considering the RWA in this scenario and using Eq.~(\ref{C_RWA}), the coefficients for the exponents are:
\begin{equation}\label{coeff_Lor_RWA}
\begin{aligned}
&\xi_{\alpha,1}^{+} = 0,~~\chi_{\alpha,1}^{+} = W-i\omega_{0},\\
&\xi_{\alpha,1}^{-} = \frac{\Gamma W}{2}, ~~\chi_{\alpha,1}^{-} = W+i\omega_{0}.
\end{aligned}
\end{equation}
These coefficients can be substituted into Eq.~(\ref{eq:HEOML_RWA}) to obtain the HEOM generator in the RWA.

\section{Diagonal decomposition of the HEOM Liouvillian superoperator}

The HEOM Liouvillian superoperator, $\hat{\mathcal{L}}_{\text{H}}$, governs the dynamics within the full ADOs space. As detailed in Eq.~(6) of the main text, this HEOM generator possesses right and left eigenmodes with the specific properties:

1. Bi-orthogonality:

~~~~~These eigenmodes, denoted by $\pmb{\rho}^{\text{L}}_j$ and $\pmb{\rho}^{\text{R}}_i$, satisfy the bi-orthogonality condition: $(\pmb{\rho}^{\text{L}}_j|\pmb{\rho}^{\text{R}}_i)=\delta_{ij}$.

2. Normalization:

~~~~~All eigenmodes can be normalized to unity: $||\hat{\pmb{\rho}}^{\text{R}}_i|| = ||\hat{\pmb{\rho}}^{\text{L}}_j|| = 1$, where $\hat{\pmb{\rho}}^{\text{R}}_i = \pmb{\rho}^{\text{R}}_i/||\pmb{\rho}^{\text{R}}_i||$ and $ \hat{\pmb{\rho}}^{\text{L}}_j = \pmb{\rho}^{\text{L}}_j/||\pmb{\rho}^{\text{L}}_j||$.

Specifically, we define the trace norm of an Auxiliary Density Operator (ADO) as:
$||\pmb{\rho}{i}^{v}|| = (\sum{k}\pmb{\rho}{i}^{v\dagger}[k]\pmb{\rho}{i}^{v}[k])^{1/2}$
where $k$ indexes elements in each eigenmode. In this formalism, both $\rho_i^L$ and $\rho_i^R$ are vectors composed of the vectorized system reduced density matrix spanned by ADOs, facilitating practical computations and analysis. Therefore, the HEOM generator admits a diagonalization:
\begin{equation}\label{eq:Reigendecom}
\hat{\mathcal{L}}_{\text{H}}=\hat{S}_{\text{R}}\hat{\Lambda}\hat{S}_{\text{R}}^{-1}.
\end{equation}
Here, the diagonal matrix $\Lambda=\text{diag}(\lambda_{0},\lambda_{1},\cdots,\lambda_{N_{\text{tot}}})$ holds the corresponding eigenvalues, while the matrix $\hat{S}_{\text{R}}$ contains the right eigenvectors $(\pmb{\rho}^{\text{R}}_{0},\pmb{\rho}^{\text{R}}_{1}\cdots \pmb{\rho}^{\text{R}}_{N_{\text{tot}}})$ as its columns. Additionally, $\hat{S}_{\text{R}}^{-1}$ represents the inverse of $\hat{S}_{\text{R}}$.
Secondly, according to the Eq.~(6), the $\hat{\mathcal{L}}_{\text{H}}$ can be diagonalized by the left eigenmodes matrix $\hat{S}_{\text{L}}=(\pmb{\rho}^{\text{L}}_{0},\pmb{\rho}^{\text{R}}_{1}\cdots \pmb{\rho}^{\text{R}}_{N_{\text{tot}}})$, resulting in:
\begin{equation}\label{eq:Leigendecom1}
\hat{S}_{\text{L}}^{\dagger}\hat{\mathcal{L}}_{\text{H}}=\hat{\Lambda}\hat{S}_{\text{L}}^{\dagger}.
\end{equation}
This translates to a diagonal decomposition of $\hat{\mathcal{L}}_{\text{H}}$:
\begin{equation}\label{eq:Leigendecom2}
\hat{\mathcal{L}}_{\text{H}}=(\hat{S}_{\text{L}}^{\dagger})^{-1}\hat{\Lambda}\hat{S}_{\text{L}}^{\dagger}.
\end{equation}
Combining Eq.~(\ref{eq:Reigendecom}) and Eq.~(\ref{eq:Leigendecom2}), we obtain the relationship:
\begin{equation}\label{eq:Leigendecom3}
\hat{S}_{\text{R}}^{-1}=\hat{S}_{\text{L}}^{\dagger}.
\end{equation}
This allows us to express the diagonal decomposition of $\hat{\mathcal{L}}_{\text{H}}$ as:
\begin{equation}\label{Leigendecom4}
\begin{aligned}
\hat{\mathcal{L}}_{\text{H}}
=\hat{S}_{\text{R}}\hat{\Lambda}\hat{S}_{\text{L}}^{\dagger}
=\sum_{i}^{N_{\text{tot}}}\lambda_{i}\pmb{\rho}^{\text{R}}_{i}\pmb{\rho}^{\text{L}\dagger}_{i}.
\end{aligned}
\end{equation}
Finally, we turn to the eigenproblem within the space of the reduced system and ADOs, where $\pmb{\rho}_{\text{s}+\text{ADO}}(t)\equiv\{\rho^{(m)}_{\bfj}(t);m=0,1\cdots,m_{\text{max}}\}$ represents the ADO vector at time $t$. The equation governing its dynamics is written as
\begin{equation}\label{eq:HEOM1}
\begin{aligned}
\frac{\partial}{\partial t}\textbf{vec}[\pmb{\rho}_{\text{s}+\text{ADO}}(t)]=\hat{\mathcal{L}}_{\text{H}}\textbf{vec}[\pmb{\rho}_{\text{s}+\text{ADO}}(t)],
\end{aligned}
\end{equation}
where $\textbf{vec}[\pmb{\rho}_{\text{s}+\text{ADO}}(t)]$ represents the vectorization of the reduced system and ADOs, facilitating the eigensolving process.
Integrating Eq.~(\ref{eq:HEOM1}) over time and utilizing the diagonal decomposition from Eq.~(\ref{eq:Leigendecom2}), we obtain
\begin{equation}\label{eq:HEOM3}
\begin{aligned}
\textbf{vec}[\pmb{\rho}_{\text{s}+\text{ADO}}(t)]&
=\exp{\left(\hat{\mathcal{L}}_{\text{H}}t\right)}\textbf{vec}[\pmb{\rho}_{\text{ini}}]\\&
=\hat{S}_{\text{R}}e^{\hat{\Lambda}t}\hat{S}_{\text{L}}^{\dagger}\textbf{vec}[\pmb{\rho}_{\text{ini}}]\\&
=\sum_{i=0}^{N_{\text{tot}}}(\pmb{\rho}^{\text{L}}_i|\textbf{vec}[\pmb{\rho}_{\text{ini}}])e^{\lambda_{i} t}\pmb{\rho}^{\text{R}}_{i}\\&
=\pmb{\rho}^{\text{R}}_{0}+\sum_{i=1}^{N_{\text{tot}}}
||\pmb{\rho}^{\text{L}}_i||
(\hat{\pmb{\rho}}^{\text{L}}_i|\textbf{vec}[\hat{\pmb{\rho}}_{\text{ini}}])
||\pmb{\rho}^{\text{R}}_i||e^{\lambda_{i} t}\hat{\pmb{\rho}}^{\text{R}}_i,
\end{aligned}
\end{equation}
where the vectorization of the initial state is represented by $\textbf{vec}[\pmb{\rho}_{\text{ini}}]$. In Eq.~(\ref{eq:HEOM3}), to achieve a trace-preserved steady state, the right eigenvectors, $\pmb{\rho}^{\text{R}}_0$, require renormalization based on the reduced density matrix. This translates to Eq.~(6) in the main text, which provides a valuable tool for investigating the unique signatures and dynamics of the non-Markovian skin effect.

\section{Non-Markovian skin effect in a Lorentzian bath}\label{nMSE_Lorentz}
\subsection{Non-Markovian memory effect}

\begin{figure}[]
	\centering
    \includegraphics[width = 1.01\columnwidth]{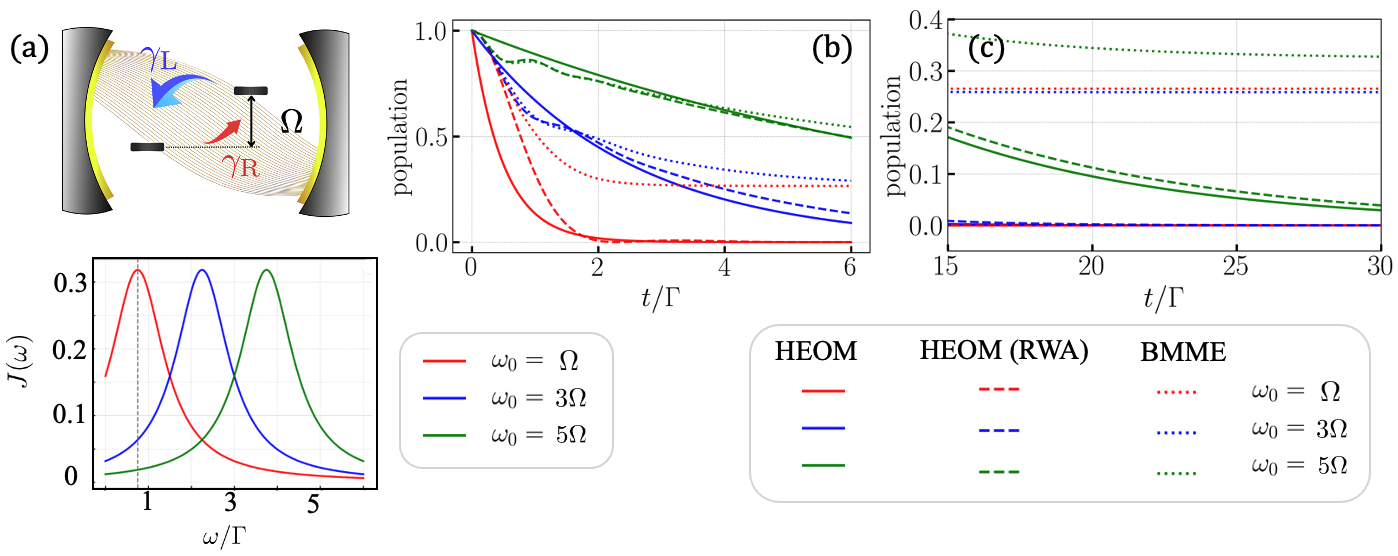}
	\caption{Illustration of non-Markovian dynamics in a Lorentzian bath. (a) Schematic representation of a two-site non-Hermitian model coupled to a bosonic bath, with left ($\gamma_L$) and right ($\gamma_R$) hopping rates and detuning $\Omega$. The lower panel shows Lorentzian spectral densities $J(\omega)$ centered at different frequencies $\omega_0$. (b) Short-time and (c) long-time evolution of the excited state population for various bath central frequencies $\omega_0$, comparing results from HEOM (solid lines), HEOM with rotating wave approximation (RWA, dashed lines), and Born-Markov master equation (BMME, dotted lines). The dynamics illustrate the impact of non-Markovian effects and virtual processes on the system evolution, particularly evident in the long-time behavior.}
	\label{N2_dynamics}
\end{figure}

The Markovian von Neumann equation describes the time evolution of a quantum system's density matrix without memory effects:
\begin{equation}
\frac{d\rho(t)}{dt} = -\frac{i}{\hbar}[H(t), \rho(t)]_{-},
\end{equation}
where $\rho(t)$ is the density matrix, $H(t)$ is the system Hamiltonian, and $[A,B]_{-} = AB - BA$ denotes the commutator.

To include memory effects, we introduce a memory kernel $K(t,t')$ that describes how the past states influence the current evolution. The resulting non-Markovian von Neumann equation, also known as the Nakajima-Zwanzig equation, takes the form:
\begin{equation}\label{nonmarkovian_correct}
\frac{d\rho(t)}{dt} = \int_0^t K(t-t')\rho(t') dt'.
\end{equation}

The integral term represents the memory effects, with $K(t-t')$ acting as a superoperator on $\rho(t')$ at earlier times $t'$. This formulation accounts for the non-Markovian nature of the system's evolution, allowing the past states to influence the current rate of change.
The memory kernel $K(t-t')$ depends on the specific properties of the system and its environment, derivable from microscopic models or phenomenological considerations. Its presence renders the equation non-local in time, reflecting the system's ability to "remember" its past states.
This non-Markovian formulation is crucial for describing open quantum systems, where the interactions with the environment lead to complex dynamics that elude simpler Markovian approximations. Fig.~\ref{N2_dynamics} illustrates the non-Markovian dynamics in a Lorentzian bath, highlighting the intricate interplay between the system and its environment.

We demonstrate that the non-Markovian memory effect can be effectively considered using the HEOM approach. To clearly illustrate this, we first examine a two-site NH model strongly interacting with a bosonic bath, which thermally induces left and right hopping terms. This model closely resembles the two-level system in a dissipative environment~\cite{HeinzPeter2016}, serving as an ideal testbed due to its simplicity and wide applicability. Such two-level systems in structured environments often exhibit memory effects, challenging Markovian approximations and revealing complex system-environment interactions.
As shown in Fig.~\ref{tau_thick_slin}, our proposed two-site NH model is described by the Hamiltonian (with $\hbar=1$ throughout):
\begin{equation}\label{H2}
H_{\text{s}}=\sum_{n=1}^{N=2}\omega_n d^\dagger_n d_n,
\end{equation}
where $d_n$ ($d_n^{\dagger}$) corresponds to the creation (annihilation) operator of the particle within the $n$th site. The bath (environment) Hamiltonian with frequency $\omega_k$ of the $k$-th mode is given by:
\begin{equation}\label{Hb}
H_{\text{b}}= \sum_k \omega_k a_k^\dagger a_k,
\end{equation}
where $a_k$ and $a_k^\dagger$ are bosonic annihilation and creation operators for the $k$-th mode of the environment. The common and well-studied system-bath interaction (I) for investigating non-Markovian physics is:
\begin{equation}\label{H2I}
H_{\text{I}} = \sum_{k}\sum_{n}g_k(a_k^{\dagger} d_{n}^{\dagger}d_{n+1}+d_{n+1}^{\dagger}d_{n} a_k),
\end{equation}
where $g_k$ is the coupling strength between the system and the $k$-th mode of the environment.
To analytically obtain the quantum dynamics of this system, we consider a Lorentzian spectral density:
\begin{equation}
J(\omega) = \frac{1}{2\pi} \frac{\Gamma W^2}{(\omega - \omega_0)^2 + W^2},
\end{equation}
where $\Gamma$ is the coupling strength between the system and the environment, $W$ is the width of the Lorentzian peak (also called the relaxation rate of the environment), and $\omega_0$ is the central frequency of the spectral density.
\begin{figure}[]
	\centering
    \includegraphics[width = 0.9\columnwidth]{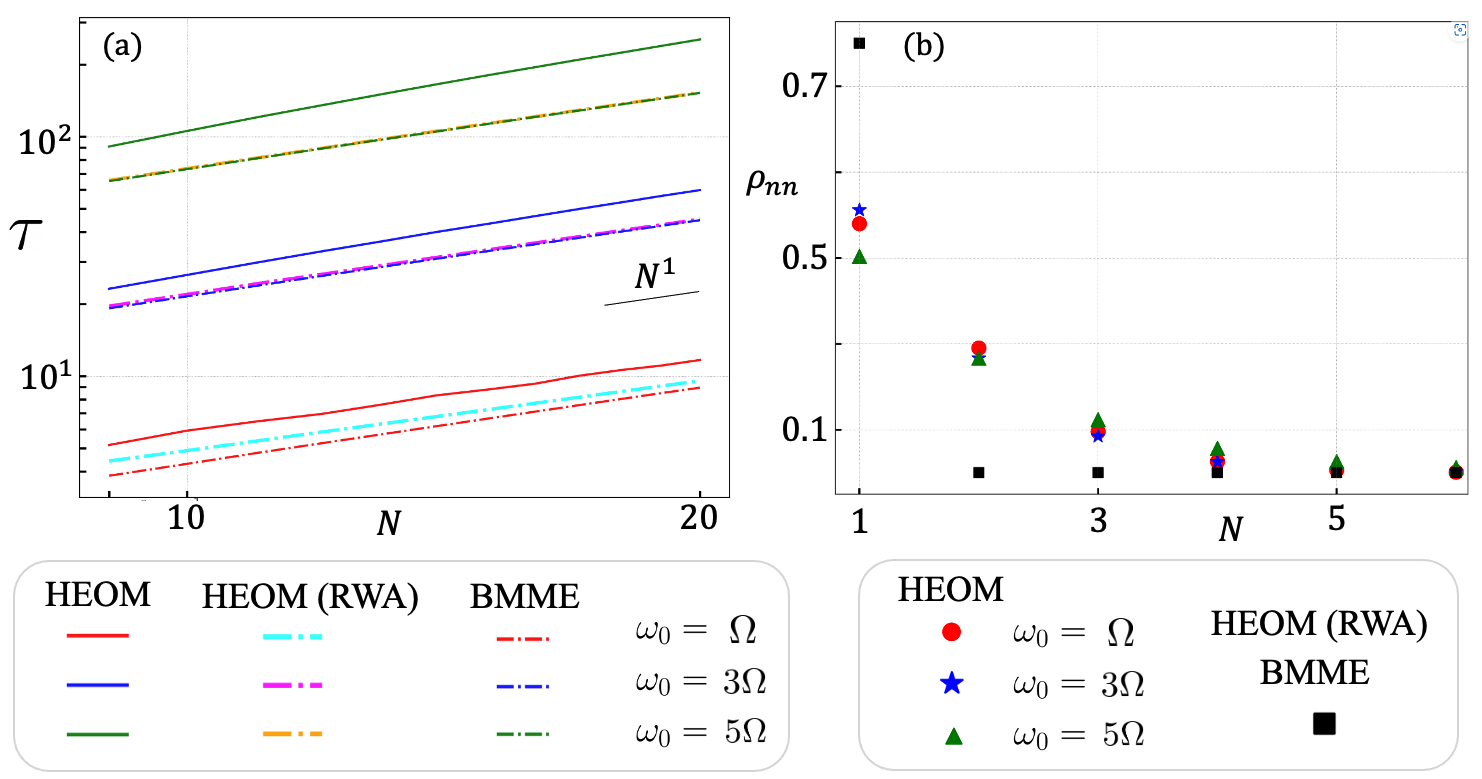}
	\caption{Illustration of the non-Markovian skin effect and thick skin effect. (a) Relaxation time $\tau$ as a function of system size $N$ for different approaches: HEOM (solid lines), HEOM with rotating wave approximation (RWA-HEOM, dash-dotted lines), and Born-Markov master equation (BMME, dash-dot-dotted lines). Results are shown for various bath central frequencies $\omega_0$ relative to system detuning $\Omega$. The black line indicates $N^1$ scaling. (b) Population distribution $\rho_{nn}$ across sites $n$ for different $N$, comparing HEOM, RWA-HEOM, and BMME approaches. The HEOM results demonstrate the thick skin effect, with population broadening into the bulk, which is absent in RWA-HEOM and BMME approaches. Both panels illustrate the crucial role of virtual processes in characterizing the non-Markovian skin effect, evident in the slower relaxation times and population distribution obtained by full HEOM calculations.}
	\label{tau_thick_slin}
\end{figure}
Additionally, we assume the temperature is at absolute zero ($k_{\text{B}}T=0$), where the hopping strength to the right, related to absorption in the Markovian limit, is zero. In this scenario, the observation of any hopping strength to the right reveals a signature of the non-Markovian effect.

Using the exact master equation via Eq.~(\ref{nonmarkovian_correct}), we can analytically solve the dynamics of this quantum system for an arbitrary initial density matrix:
\begin{equation}\label{rho0}
\rho_{\text{s}}(0)=
\begin{pmatrix}
1 - \alpha_{\text{s}} & \beta_{\text{s}} \\
\beta_{\text{s}}^{\ast} & \alpha_{\text{s}}
\end{pmatrix}
\end{equation}
Notably, we can also perform the diagonal decomposition of HEOM with RWA via Eq.~(\ref{eq:HEOM3}) to obtain the exact system dynamics and reveal the non-Markovian memory effect exhibited in Eq.~(\ref{nonmarkovian_correct}). For spectral analysis, we consider the vectorized representation of the HEOM:
\begin{equation}
    \begin{aligned}
    \frac{d}{dt}\textbf{vec}[\rho_{\s+\ADO}(t)]= \mathcal{L}^{\text{RWA}}_{\s+\ADO}\textbf{vec}[\rho_{\s+\ADO}(t)],
    \end{aligned}
\end{equation}
where $\mathcal{L}^{\text{RWA}}_{\s+\ADO}$ is given by Eq.~(\ref{eq:HEOML_RWA}) and the encoded bath correlation is referred to that in Eq.~(\ref{coeff_Lor_RWA}).
\begin{figure}[]
	\centering
    \includegraphics[width = 0.83\columnwidth]{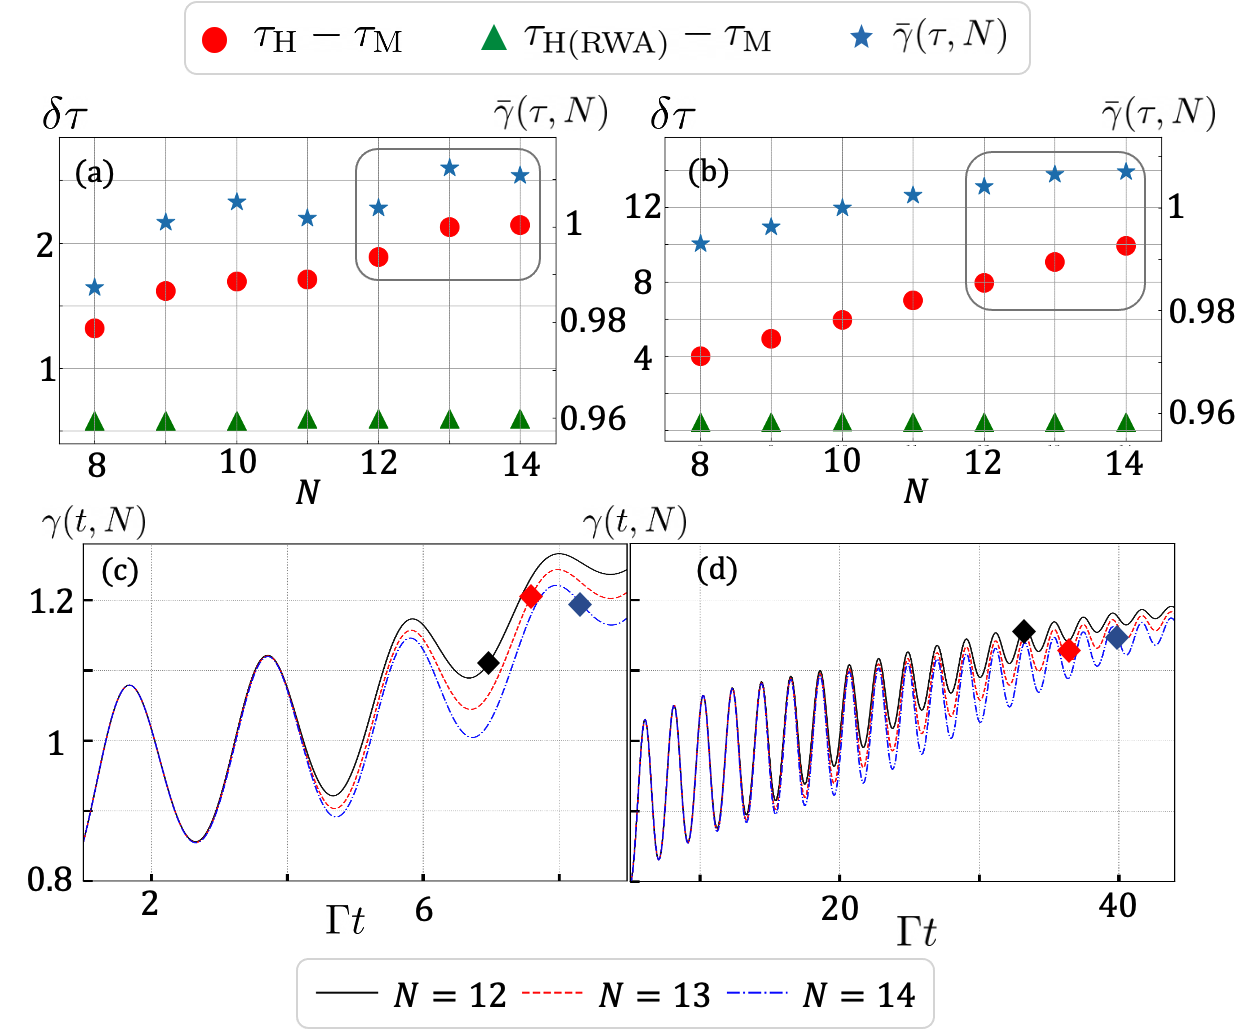}
	\caption{Oscillatory behavior in the relaxation time $\tau$ and the scaled rate of particle transport $\bar{\gamma}(t,N)$. (a,b) Comparison of relaxation time differences $\delta\tau$ between HEOM and BMME ($\tau_H - \tau_M$, red circles), HEOM with RWA and BMME [$\tau_{H(RWA)} - \tau_M$, green triangles], and the average scaled rate of particle transport $\bar{\gamma}(\tau,N)$ (blue stars) as functions of system size $N$ for (a) $\omega_0 = \Omega$ and (b) $\omega_0 = 3\Omega$. (c,d) Time evolution of $\gamma(t,N)$ for $N=12, 13,$ and $14$ when (c) $\omega_{0}=\Omega$ and (d) $\omega_{0}=3\Omega$. Markers indicate the relaxation time points. The oscillatory behavior of $\gamma(t,N)$ leads to the oscillatory-like trend in $\delta\tau$ and $\bar{\gamma}(\tau,N)$ with respect to $N$, demonstrating the connection between system coherence and relaxation dynamics in the non-Markovian regime.}
	\label{tau_oscillation}
\end{figure}

Due to the absence of the internal tunneling between the two sites, the system's behavior can be accurately captured by considering up to the second hierarchical tier ($m=2$)~\cite{exactruncation2018}. This truncation's validity can be further verified using Eq.~(\ref{nonmarkovian_correct}). The corresponding extended Liouvillian superoperator is represented as a $24\times24$ matrix. To facilitate the analytical calculations, we decompose $\mathcal{L}_{\text{S}+\text{ADO}}^{\text{RWA}}$ into three components:
\begin{equation}
\begin{aligned}
\mathcal{L}_{\text{s}+\text{ADO}}^{\text{RWA}}
=\mathcal{L}_{\text{s}+\text{ADO}}^{\text{RWA},\text{p}}
\oplus\mathcal{L}_{\text{s}+\text{ADO}}^{\text{RWA},\text{c}}
\oplus\mathcal{L}_{\text{s}+\text{ADO}}^{\text{RWA},\text{c}\ast},
\label{eq:HEOML_RWA2}
\end{aligned}
\end{equation}
where the superscripts p, c, and $\text{c}\ast$ indicate the components determining the system's population, coherence, and its complex conjugate, respectively. The full expressions for these components are:
\begin{equation}
\begin{aligned}
\mathcal{L}_{\text{s}+\text{ADO}}^{\text{RWA},\text{p}}=
\begin{pmatrix}
0 & 0 & -i & i & 0 & 0 \\
0 & 0 & i & -i & 0 & 0 \\
0 & i W \Gamma/2 & -W + i (\omega_{0}-\Omega) & 0 & -i & i \\
0 & -i W \Gamma/2 & 0 & -W + i (\Omega - \omega_{0}) & i & -i \\
0 & 0 & -i W \Gamma/2 & i W \Gamma/2 & -2W & 0 \\
0 & 0 & 0 & 0 & 0 & -2W
\end{pmatrix},
\end{aligned}
\end{equation}
\begin{equation}
\begin{aligned}
\mathcal{L}_{\text{s}+\text{ADO}}^{\text{RWA},\text{c}}=
\begin{pmatrix}
-i \Omega & -i & i & 0 & 0 \\
-i W \Gamma/2 & -W - i \omega_{0} & 0 & -i & i \\
0 & 0 & -W - i \omega_{0} & i & -i \\
0 & 0 & i W \Gamma/2 & -2W - i \Omega & 0 \\
0 & 0 & -i W \Gamma/2 & 0 & -2W + i (\Omega - 2 \omega_{0})
\end{pmatrix},
\end{aligned}
\end{equation}
\begin{equation}
\begin{aligned}
\mathcal{L}_{\text{s}+\text{ADO}}^{\text{RWA},\text{c}\ast}=
\begin{pmatrix}
i \Omega & i & -i & 0 & 0 \\
i W \Gamma/2 & -W + i \omega_{0} & 0 & -i & i \\
0 & 0 & -W + i \omega_{0} & i & -i \\
0 & 0 & i W \Gamma/2 & -2W - i (\Omega - 2 \omega_{0}) & 0 \\
0 & 0 & -i W \Gamma/2 & 0 & -2W + i \Omega
\end{pmatrix},
\end{aligned}
\end{equation}
where the detuning $\Omega=\omega_{2}-\omega_{1}$.

By performing the diagonal decomposition of each extended Liouvillian superoperator according to Eq.~(\ref{Leigendecom4}), we obtain the corresponding left and right eigenmodes. These eigenmodes allow us to construct the complete quantum dynamics via Eq.~(\ref{eq:HEOM3}). We label the elements of the system density matrix and its vectorized version as:
\begin{equation}
\begin{aligned}
\rho_{\text{s}}(t)=
\begin{pmatrix}
\rho_{11}(t) & \rho_{12}(t) \\ 
\rho_{21}(t) & \rho_{22}(t) \\ 
\end{pmatrix},\text{~~~and~~~}
\textbf{vec}[\rho_{\text{s}}(t)]=
\begin{pmatrix}
\rho_{11}(t) \\ 
\rho_{21}(t) \\ 
\rho_{12}(t) \\
\rho_{22}(t) \\
\end{pmatrix},
\end{aligned}
\end{equation}
Analytically solving Eq.~(\ref{eq:HEOM3}) using $\mathcal{L}_{\text{s}+\text{ADO}}^{\text{RWA},\text{p}}$, $\mathcal{L}_{\text{s}+\text{ADO}}^{\text{RWA},\text{c}}$, and $\mathcal{L}_{\text{s}+\text{ADO}}^{\text{RWA},\text{c}\ast}$, we obtain the population of the second site and the coherence terms:
\begin{equation}\label{rho22}
\rho_{22} = \alpha_{\text{s}} |G(t)|^2,~~~~\rho_{12} = \beta_{\text{s}}G(t)\text{,~~ and}~~~~\rho_{21} = \beta_{\text{s}}^{\ast}G(t)^{\ast},
\end{equation}
where 
\begin{equation}\label{G}
G(t) = \left\{ \cosh\left[t\sqrt{W(W - 2\Gamma)}/2\right] + \sqrt{W/(W - 2\Gamma)} \sinh\left[t\sqrt{W(W - 2\Gamma)}/2\right] \right\}\exp\left[\frac{-t(W - 2i\Omega)}{2}\right] .
\end{equation}
Here, $\Omega$ represents the detuning $(\omega_2-\omega_1)$. This analytical solution is consistent with results obtained from Eq.~(\ref{nonmarkovian_correct}), demonstrating that the diagonal decomposition of the HEOM Liouvillian superoperator accurately captures the non-Markovian memory effect.
\begin{figure}[]
	\centering
    \includegraphics[width = \columnwidth]{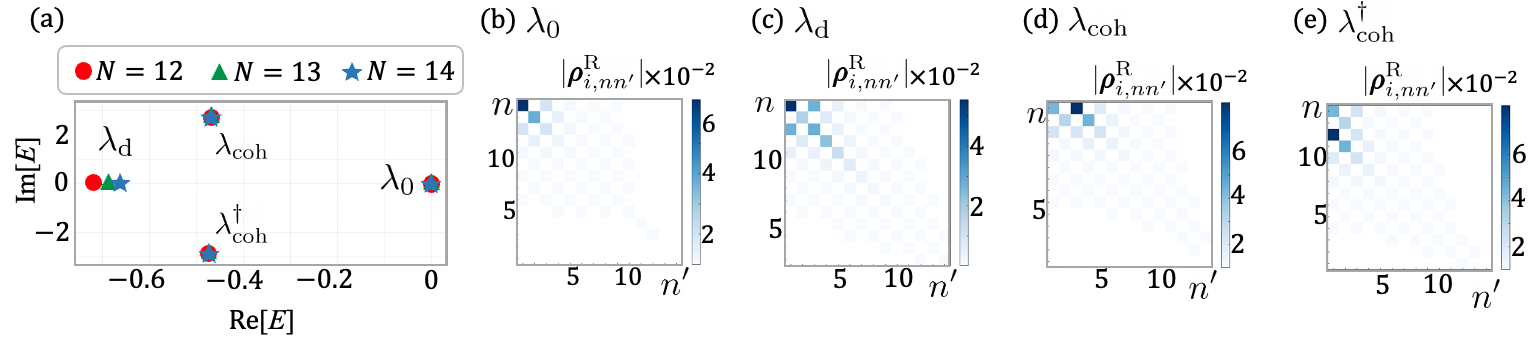}
	\caption{Eigenspectrum analysis of the non-Markovian dynamics. (a) Eigenvalue distribution in the complex plane for systems with $N=12, 13,$ and $14$ sites, showing steady state ($\lambda_0$), skin mode ($\lambda_d$), and secondary skin modes ($\lambda_{\text{coh}}$, $\lambda_{\text{coh}}^{\dagger}$) eigenvalues. (b-e) Absolute values of the reduced density matrices $|\rho_{i,nn'}^R|$ for (b) steady state $\hat{\pmb{\rho}}_{\text{ss}}$, (c) skin mode $\hat{\pmb{\rho}}_{\text{d}}$, and (d,e) secondary skin modes $\hat{\pmb{\rho}}_{\text{coh}}$ and $\hat{\pmb{\rho}}_{\text{coh}}^{\dagger}$. The presence of imaginary parts in $\lambda_{\text{coh}}$ and $\lambda_{\text{coh}}^{\dagger}$ contribute to oscillations in $\gamma(t,N)$, while their proximity to $\lambda_0$ allows for persistent coherence effects.}
	\label{eig_spectrum_N}
\end{figure}

To investigate how the non-Markovian effect influences the system dynamics, we engineer the spectral density of the strongly coupled bath by adjusting the central frequency $\omega_{0}$ to be resonant or off-resonant with the two-site detuning $\Omega$ (Fig.~\ref{N2_dynamics}). Compared to the BMME approach, when $\omega_{0}$ is resonant with $\Omega$, the non-Markovian effect delays the evolution of the two-site system. The presence of memory effects leads to complex, non-exponential decay of correlations, generally slowing down the overall dynamics compared to Markovian systems. However, as the system's transition frequency $\omega_{0}$ deviates further from the bath's characteristic frequency $\Omega$, the non-Markovian nature of the system manifests as more pronounced oscillations in the short-time regime. This results in a counterintuitive acceleration of the relaxation process, a phenomenon that can also be understood within the framework of the anti-Zeno effect~\cite{JhenDong2022}. This allows us to manipulate the speed difference between Markovian and non-Markovian dynamics through the environmental engineering.

\subsection{Virtual processes in the strong coupling regime}

It is important to note that the above considerations do not account for the virtual processes described by the counter-rotating terms. To include these terms, we use the general version of HEOM, Eq.~(\ref{eq:HEOML}), and express the vectorized representation as:
\begin{equation}
    \begin{aligned}
    \frac{d}{dt}\textbf{vec}[\rho_{\s+\ADO}(t)]= \mathcal{L}_{\s+\ADO}\textbf{vec}[\rho_{\s+\ADO}(t)],
    \end{aligned}
\end{equation}
Including the virtual processes requires higher tiers of HEOM, significantly increasing the dimensions of the HEOM Liouvillian superoperator and precluding simple analytical forms. Therefore, we present numerical results of non-Markovian dynamics in Fig.~\ref{N2_dynamics}. Interestingly, the virtual processes minimally affect the short-time dynamics but significantly influences the long-term behavior, maintaining excitation in the excited state (second site population). This substantially impacts the long-time behavior, particularly the skin effect dominated by non-Markovian dynamics.
As we extend the number of sites to $N$ in the coupled environment structure (at zero temperature), we observe the signature of the non-Markovian skin effect, as shown in Fig.~\ref{tau_thick_slin}(a). Regardless of how the bath structure or parameters are engineered to alter non-Markovian dynamics in short-time behavior, the non-Markovian skin effect, dominated by the long-time behavior, reveals a consistent system relaxation property: the relaxation time $\tau$ is proportional to the system size $N$.

In fact, the virtual processes are crucial for characterizing a particular aspect of the non-Markovian skin effect. Firstly, the $\tau$ obtained by HEOM is significantly slower than that those obtained by RWA HEOM and BMME, with the difference becoming more pronounced for larger system sizes. Moreover, without the virtual processes, there is no thick skin effect at all, as demonstrated in Fig.~\ref{tau_thick_slin}(b). Even though the HEOM approach with RWA includes the non-Markovian effect, it cannot present the thick skin effect. Different bath parameters, such as varying central frequencies, also exhibit the thick skin effect, causing population broadening into the bulk.
To investigate whether the non-Markovian effect induces oscillatory behavior in the relaxation time $\tau$ with respect to the number of sites, we analyze the difference in relaxation time between HEOM and BMME, $\delta\tau=\tau_{\text{H}}-\tau_{\text{M}}$, as shown in Fig.~\ref{tau_oscillation}. For comparison with the virtual processes, we also examine the difference in relaxation time between RWA HEOM and BMME, $\delta\tau=\tau_{\text{H(RWA)}}-\tau_{\text{M}}$. We compare $\delta\tau$ with the average scaled rate of particle transport $\bar{\gamma}(\tau,N)$, which describes the summation of cumulated coherence.

As the site number increases, $\delta\tau$ (i.e., $\tau_{\text{H(RWA)}}-\tau_{\text{M}}$) follows the same trend as $\bar{\gamma}(\tau,N)$, regardless of how the bath central frequency $\omega_{0}$ is tuned. As $\omega_{0}$ shifts from resonant with $\Omega$ to $3\Omega$, the oscillatory behavior of the relaxation time $\tau$ disappears and monotonically increases with respect to $N$. Simultaneously, $\bar{\gamma}(\tau,N)$ exhibits smooth and monotonic behavior, further demonstrating that the oscillation in the relaxation time $\tau$ is related to the variation of the system coherence.
The key mechanism behind the oscillatory $\bar{\gamma}(\tau,N)$ with respect to $N$ is the significant oscillatory behavior of the scaled rate of particle transport $\gamma(t,N)$, as shown in Fig.~\ref{tau_oscillation}(c). To obtain $\bar{\gamma}(\tau,N)$, we integrate $\gamma(t,N)$ with the upper limit $\tau$ for each different $N$ and then average over time divided by $\tau$. For example, with $N=12, 13,$ and $14$, the relaxation time point on $\gamma(t,N)$ is located near the dip, peak, and dip again, respectively. This oscillation with significant amplitude in $\gamma(t,N)$ results in the oscillatory-like behavior of the relaxation time with respect to neighboring sites.
When $\omega_{0}=5\Omega$, $\bar{\gamma}(\tau,N)$ increases monotonically. Although the corresponding $\gamma(t,N)$ still exhibits oscillations, its amplitude is relatively small and barely detectable in $\bar{\gamma}(\tau,N)$.
\begin{figure}[]
	\centering
    \includegraphics[width = 1.0\columnwidth]{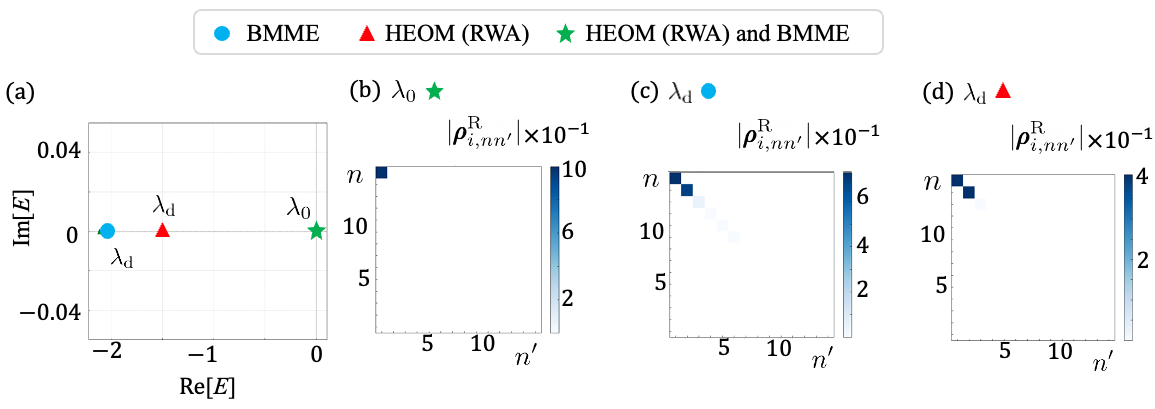}
	\caption{Eigenspectrum analysis of the HEOM Liouvillian superoperator under the RWA. (a) Eigenvalue distribution in the complex plane for BMME, RWA-HEOM, and their overlap, showing only real eigenvalues. (b-d) Absolute values of the reduced density matrices $|\rho_{i,nn'}^R|$ for (b) steady state $\hat{\pmb{\rho}}_{\text{ss}}$, (c) BMME skin mode, and (d) RWA-HEOM skin mode. The absence of imaginary eigenvalues and coherence in these modes demonstrates that virtual processes are crucial for observing oscillations in $\gamma(t,N)$ and relaxation time.}
	\label{eig_spectrum_ME_RWA}
\end{figure}
To elucidate the influence of the eigenmodes on the oscillations of $\gamma(t,N)$, we analyze the eigenspectrum of the Liouvillian for systems for $N=12, 13,$ and $14$ sites. As shown in Fig.~\ref{eig_spectrum_N}(a), we observe not only the steady state $\hat{\pmb{\rho}}_{\text{ss}}$ (corresponding to zero eigenvalue $\lambda_0$) and the skin mode $\hat{\pmb{\rho}}_{\text{d}}$ (with eigenvalue $\lambda_\text{d}$), but also two additional secondary skin modes that play a crucial role in determining the non-Markovian long-time behavior of the relaxation time.
These secondary skin modes, $\hat{\pmb{\rho}}_{\text{coh}}$ and $\hat{\pmb{\rho}}_{\text{coh}}^{\dagger}$, have eigenvalues $\lambda_{\text{coh}}$ and $\lambda_{\text{coh}}^{\dagger}$ with imaginary parts. The real parts of these eigenvalues are closer to the steady state than the skin mode, allowing these eigenmodes to persist longer in the long-term behavior. Analysis of these dominant eigenmodes reveals that $\hat{\pmb{\rho}}_{\text{d}}$, $\hat{\pmb{\rho}}_{\text{ss}}$, $\hat{\pmb{\rho}}_{\text{coh}}$, and $\hat{\pmb{\rho}}_{\text{coh}}^{\dagger}$ all exhibit significant coherence, as illustrated in Fig.~\ref{eig_spectrum_N}(b).

Intuitively, $\hat{\pmb{\rho}}_{\text{coh}}$ and $\hat{\pmb{\rho}}_{\text{coh}}^{\dagger}$ are conjugate pairs that substantially contribute to the oscillations of $\gamma(t,N)$, with their imaginary parts driving coherence oscillations. Furthermore, the smaller real part of the skin mode eigenvalue for larger system sizes contributes to the long-term coherence behavior, as all these eigenmodes, including the skin mode, contribute to system coherence in the non-Markovian dynamics.

Interestingly, when analyzing the eigenspectrum of the HEOM Liouvillian superoperator with RWA (Fig.~\ref{eig_spectrum_ME_RWA}(a)), we observe only dominant eigenmodes with purely real eigenvalues. However, these eigenvalues are closer to zero compared to the Liouvillian gap obtained from BMME, indicating that the non-Markovian effects can slow down the dynamics relative to Markovian ones.
Extraction and analysis of all contributing eigenmodes, including $\hat{\pmb{\rho}}_{\text{ss}}$ and $\hat{\pmb{\rho}}_{\text{d}}$ for both HEOM with RWA and BMME, reveal no coherence in the eigenmodes. This suggests that even when considering the non-Markovian effects in the skin effect, the absence of virtual processes precludes the observation of the coherence, oscillations in $\gamma(t,N)$, and oscillations in relaxation time as a function of $N$.

\section{Collective and separated couplings to the bath for the non-Markovian skin effect}

\begin{figure}[]
	\centering
    \includegraphics[width = 1\columnwidth]{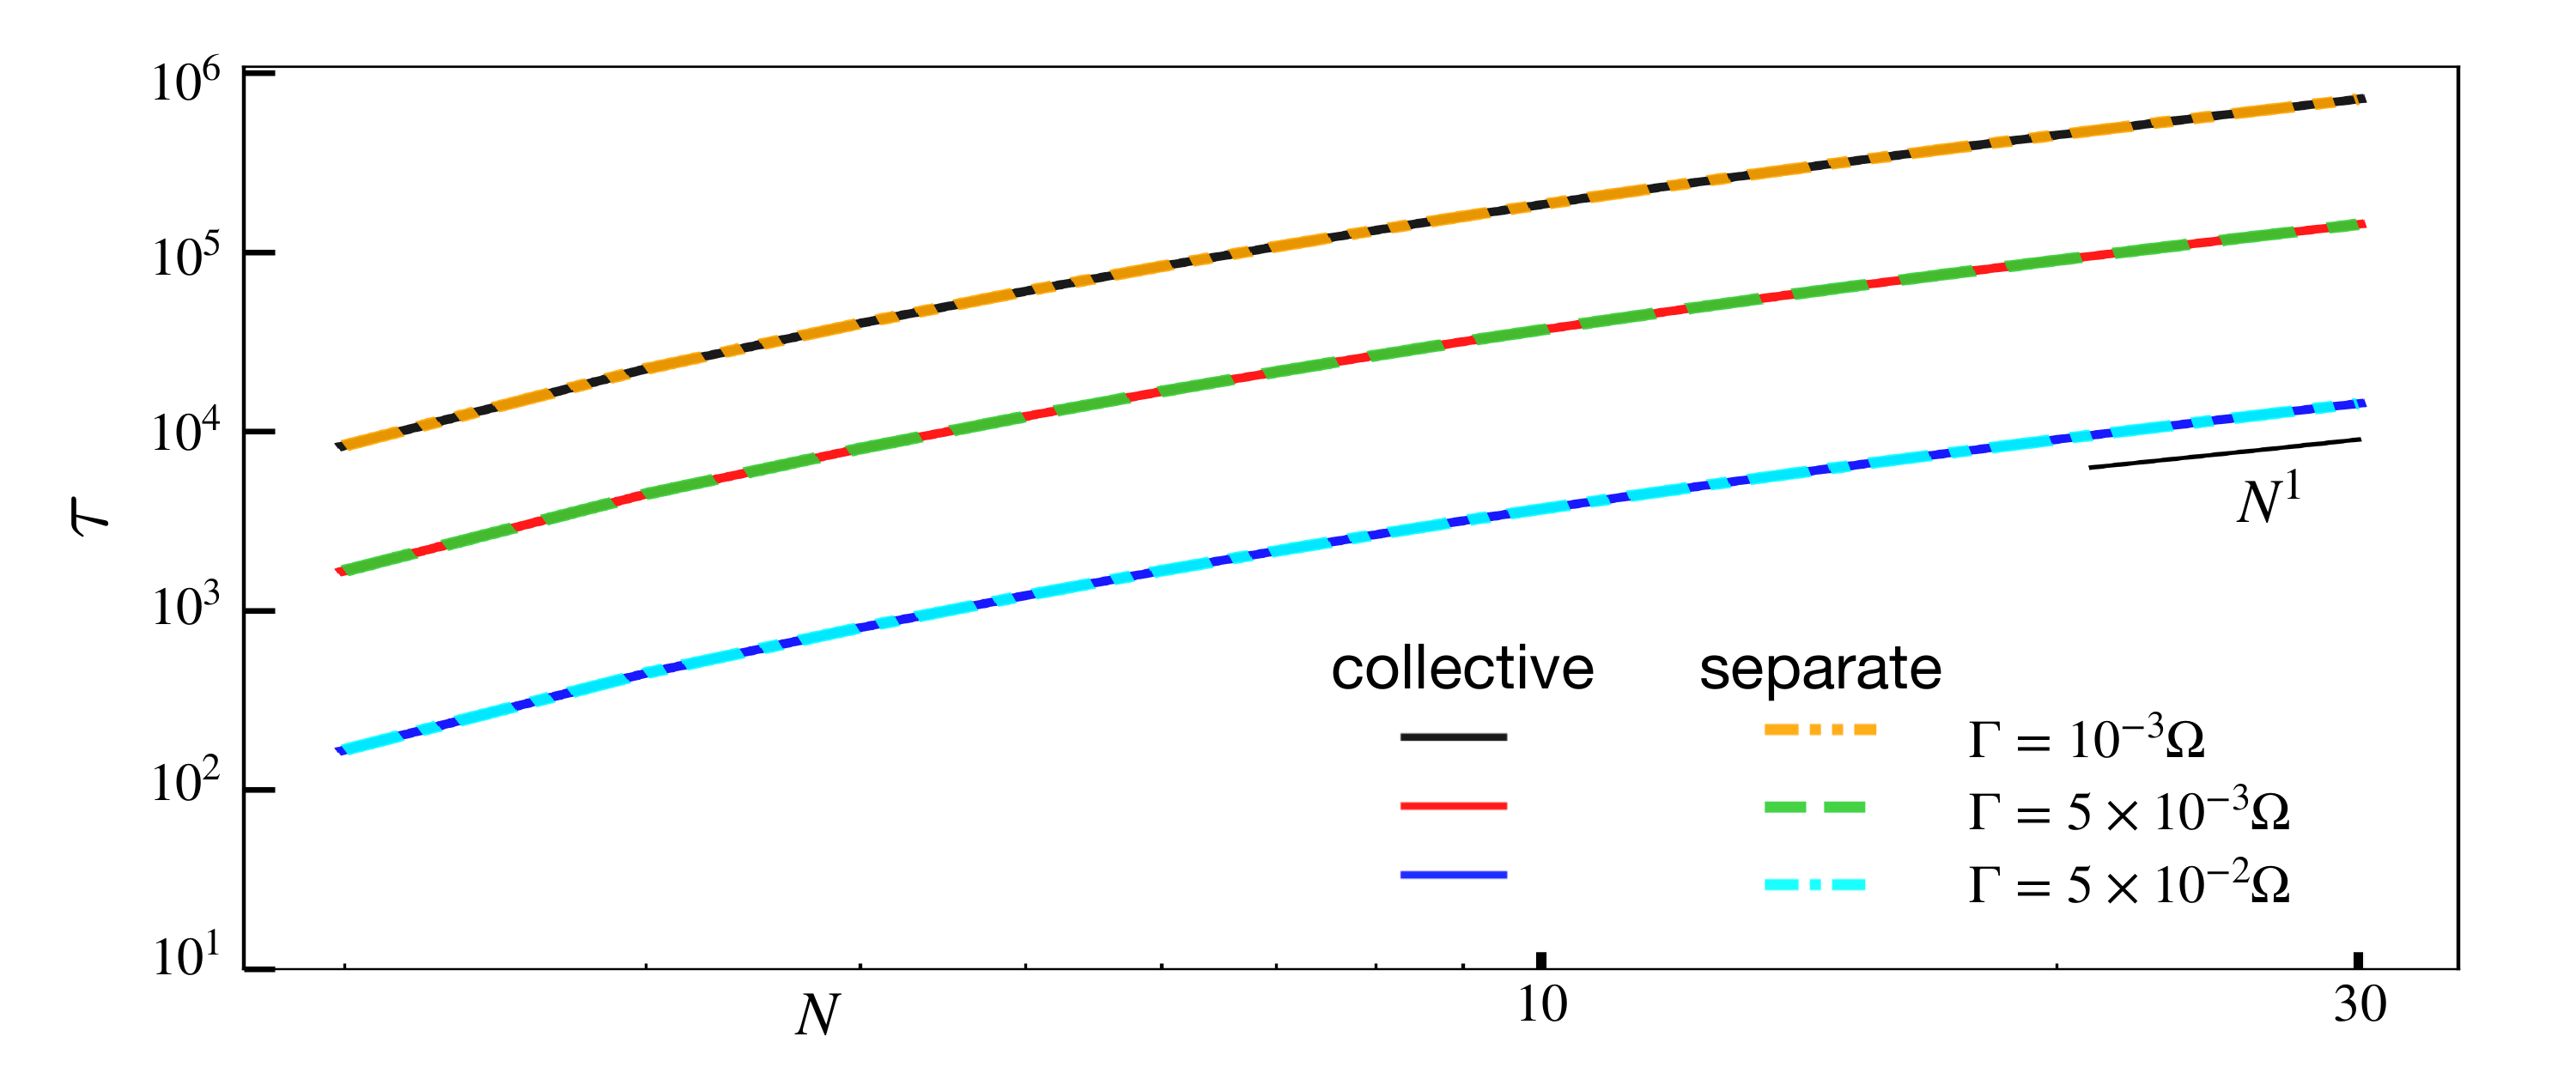}
	\caption{Relaxation time $\tau$ as a function of $N$, calculated using the Born-Markov master equation (BMME) under collective (solid curves) and separate (dashed curves) coupling conditions for various coupling strengths: $\Gamma=10^{-3},5\times10^{-3}$, and $5\times10^{-2}\Omega$. The short black line segment on the right indicates a linear $(N^1)$ scaling behavior.  Both axes are plotted in logarithmic scales.}
	\label{fig:ME}
\end{figure}

This section focuses on the non-Markovian Liouvillian skin effect (LSE) in a specific limit: a one-dimensional chain where sites are far apart and each hopping between neighboring sites is driven by independent (separated) baths. In this configuration, each adjacent pair of sites within the $N$-site lattice is coupled to an individual environment, resulting in a total of $(N-1)$ baths. Under the Markovian regime with small coupling strength $\Gamma$, investigations of the Liouvillian skin effect predominantly rely on the Born-Markov approximation. This approximation is characterized by the Markovian Liouvillian $\mathcal{L}_{\text{M}}[\cdot]$ in the Born-Markov master equation (BMME):
\begin{equation}
\begin{aligned}
    \mathcal{L}_{\text{M}}[\rho_{\text{s}}]=\mathcal{L}_{0}[\rho_{\text{s}}]+\sum_{\alpha}\left(L_{\alpha}\rho_{\text{s}}L_{\alpha}^{\dagger}-\frac{1}{2}[L_{\alpha}^{\dagger}L_{\alpha},\rho_{\text{s}}]_{+}\right).\label{eq:Master eq}
\end{aligned}
\end{equation}
Here, $\mathcal{L}_{0}[\cdot]=-i[H_{\text{s}},\cdot]_{-}$ incorporates the system Hamiltonian $H{\text{s}}$, with $[\cdot,\cdot]_{-}$ and $[\cdot,\cdot]_{+}$ denoting the commutator and anticommutator, respectively. The crucial nonreciprocal hopping operators characterizing the LSE are defined as
\begin{equation}\label{eq:liouvillian separated}
    L_{\text{L},n}=\sqrt{\gamma_{\text{L}}}~d_{n}^{\dagger}d_{n+1}, 
    \:  \: \:
    L_{\text{R},n}=\sqrt{\gamma_{\text{R}}}~d_{n+1}^{\dagger}d_{n},
\end{equation}
where $L_{\text{L},n}$ and $L_{\text{R},n}$ represent the leftward and rightward hopping operators for site $n$, $\gamma_{\text{L},n}$ and $\gamma_{\text{R},n}$ denote the associated left and right coupling constants, and $d_{n}$ and $d_{n}^{\dagger}$ are the annihilation and creation operators for the particle state at site $n$. Based on the BMME, the Liouvillian for this separate-bath configuration can be written as
\begin{equation}\label{eq:liouvillian separated}
    \mathcal{L}_{\text{M}(\text{s})}[\rho_{\text{s}}]= 
    \mathcal{L}_{0}[\rho_{\text{s}}]+
    \sum_{n=1}^{N-1}\sum_{v=\text{L},\text{R}}
    \left(L_{v,n}\rho_{\text{s}}L_{v,n}^{\dagger}-\frac{1}{2}[L_{v,n}^{\dagger}L_{v,n},\rho_{\text{s}}]_{+}\right),
\end{equation}
where $\mathcal{L}_{0}$ denotes the free system evolution, $v$ indexes over the left and right hopping directions, and $[\cdot,\cdot]_{+}$ represents the anti-commutator.

\begin{figure}[]
	\centering
    \includegraphics[width = .48\columnwidth]{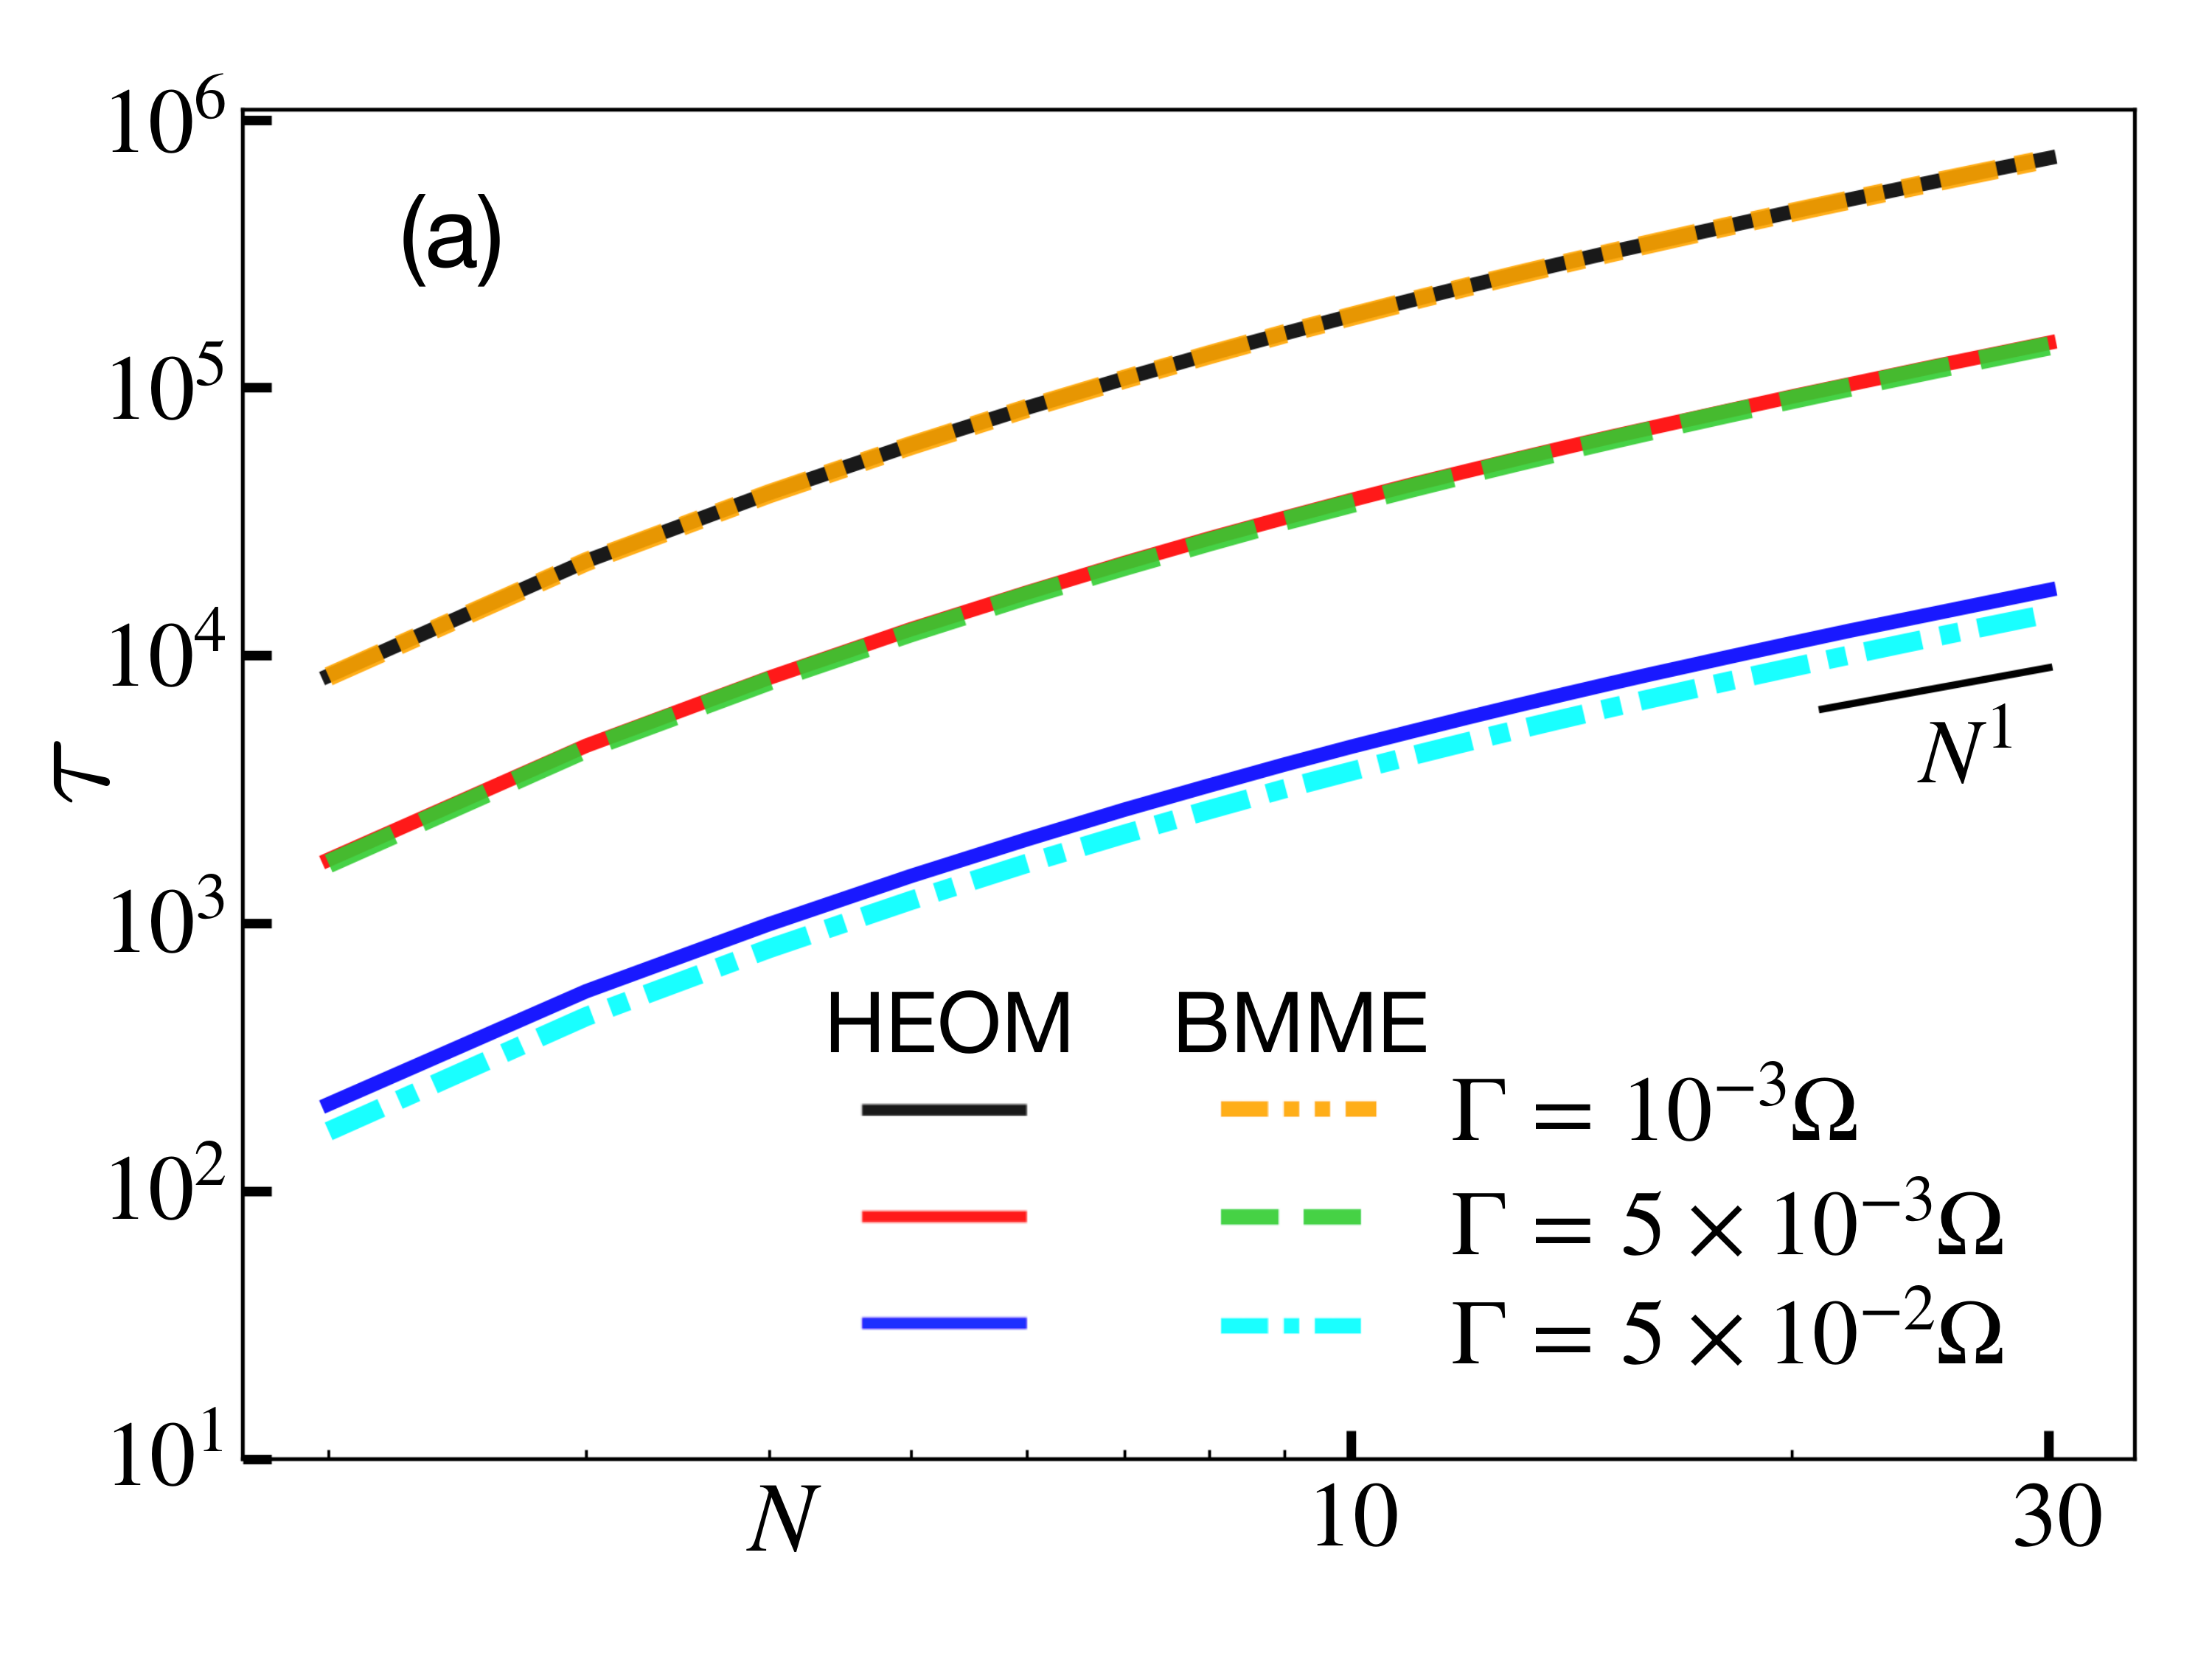}
    \hspace{0.1in}
    \includegraphics[width = .48\columnwidth]{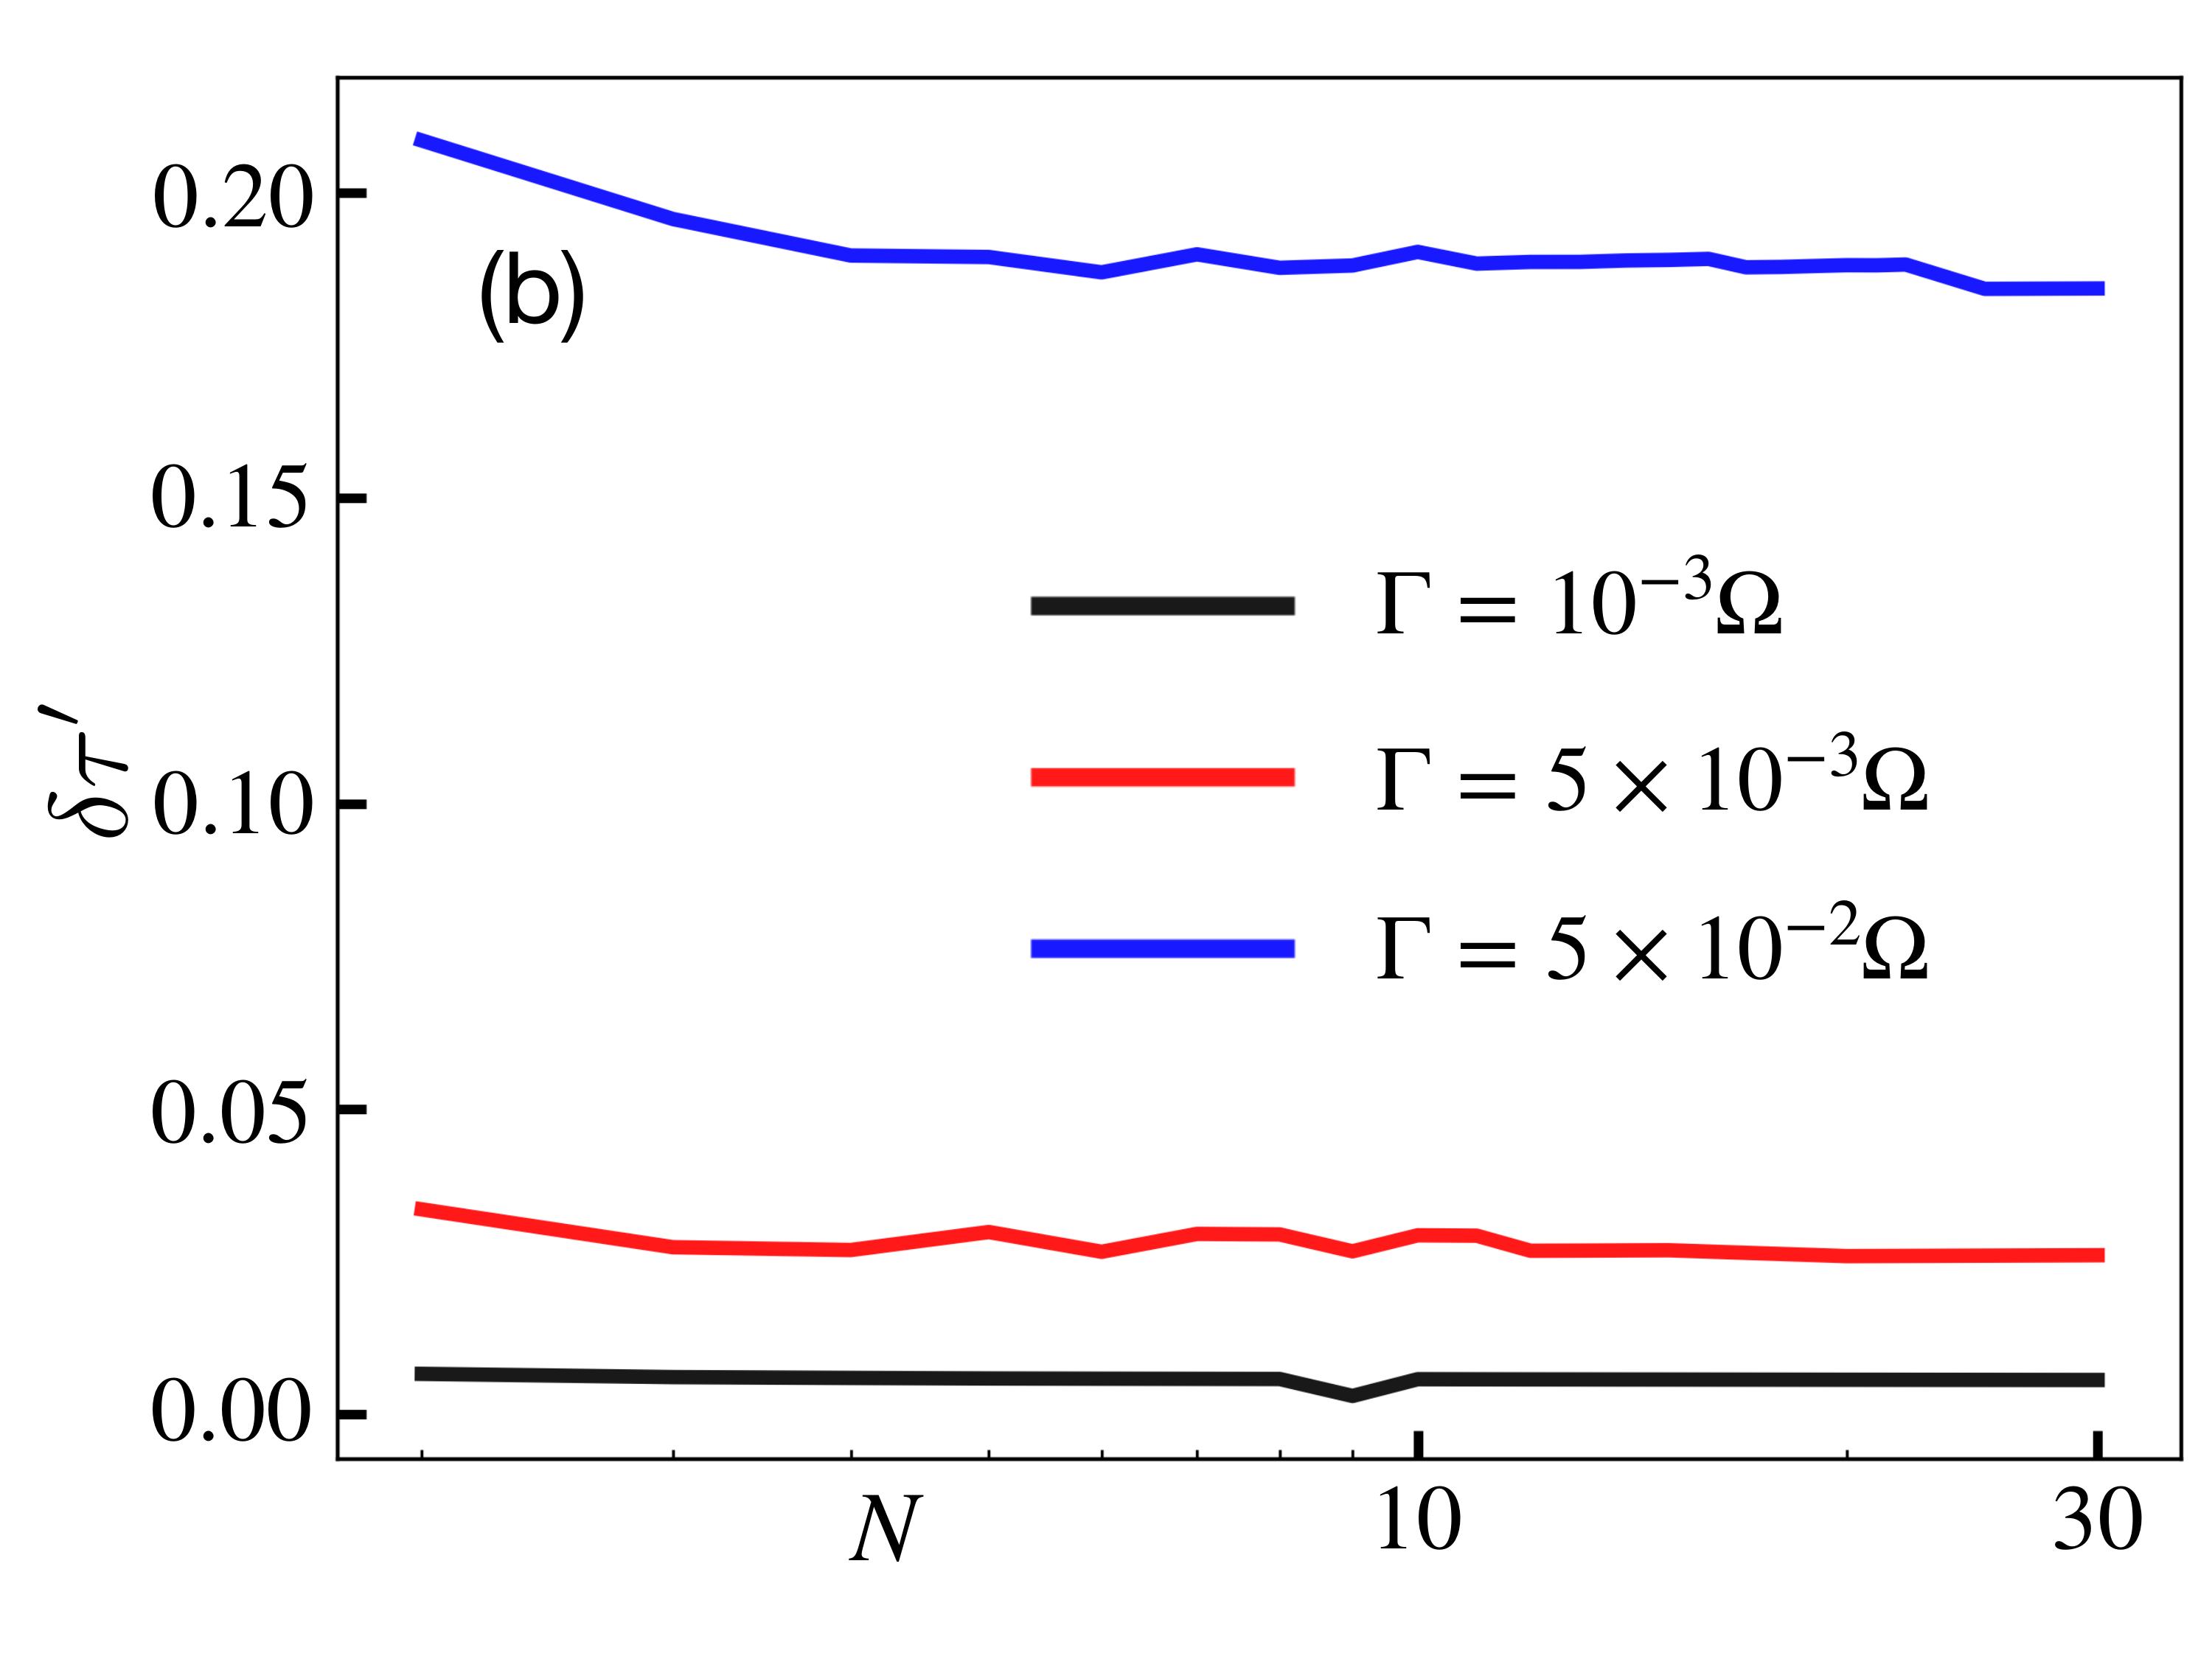}
	\caption{(a) Relaxation time $\tau$ for the collective coupling plotted against $N$ in both Markovian (dashed curves) and non-Markovian (solid curves) regimes for different coupling strengths: $\Gamma=10^{-3},5\times10^{-3}$, and $5\times10^{-2}\Omega$. The black line represents a linear, $N^1$, scaling. Both axes are in logarithmic scale. (b) Ratio of relaxation time differences between HEOM, $\tau_{\text{H}}$, and BMME, $\tau_{\text{M}}$, quantified as $(\tau_{\text{H}}-\tau_{\text{M}})/\tau_{\text{H}}$, as a function of $N$ for different coupling strength $\Gamma$. The horizontal axis is in logarithmic scale.}
	\label{fig:deltatau}
\end{figure}

\begin{figure}[]
	\centering
    \includegraphics[width = 1.\columnwidth]{figS3.pdf}
	\caption{Eigenenergy ($E$) distributions for the dominant evolution modes calculated by HEOM (red dots) and BMME (blue dots) for different coupling strengths: $\Gamma=10^{-3},5\times10^{-3}$, and $5\times10^{-2}\Omega$. This comparison highlights the divergence in eigenenergy spectra with increasing coupling strength, specifically focusing on the most impactful modes governing system dynamics.}
	\label{fig:eigen}
\end{figure}

Comparing our one-dimensional chain with the setup of collective coupling to a shared bath reveals a key finding: both systems exhibit the Liouvillian skin effect (LSE) regardless of the bath coupling configuration (collective vs. separate coupling). 

Analyzing the relaxation time, $\tau$, as a function of the number $N$ of sites in both models (initially prepared in $\rho_{\text{ini}}=\ket{N}\bra{N}$), using the Born-Markov master equation (Fig.~\ref{fig:ME}) to represent the Markovian regime, further supports this observation. Under this framework, the specific bath coupling configurations (collective versus separate) become indistinguishable in their influence on the observed long-time dynamics, as reflected by their identical behavior in the LSE regime. Both models exhibit a consistent linear scaling of the relaxation time with increasing system size.

While the results in the main text have extensively explored the model with collective bath coupling, which exhibits rich phenomenology, we now turn our attention to the system with separated bath interactions to provide a more complete picture.

Entering the non-Markovian regime through increasing $\Gamma$ and utilizing HEOM with the system interaction operator $V_{\Symbol{\sigma}{b},n} = d_{n}^{\dagger}d_{n+1} + d_{n+1}^{\dagger}d_{n}$ reveals a striking divergence in relaxation times compared to the Markovian regime (Fig.~\ref{fig:deltatau}). This direct observation signifies that the non-Markovian effects noticeably slow down the system's dynamics, leading to a longer relaxation time. This slowdown offers significant insights into the interplay between system-bath interactions and temporal evolution in the non-Markovian domain.

To quantify the impact of non-Markovian effects on relaxation, we define a ratio of relaxation time differences, $\delta\tau'$, between the HEOM and BMME time scales
\begin{equation}
\delta\tau' = \frac{\tau_{\text{H}} - \tau_{\text{M}}}{\tau_{\text{H}}},
\end{equation}
where $\tau_{\text{H}}$ and $\tau_{\text{M}}$ represent the relaxation times obtained using the HEOM and BMME methods, respectively. As shown in Figure~\ref{fig:deltatau}, $\delta\tau'$ exhibits a progressive enhancement when increasing the coupling strength, $\Gamma$. This signifies a significant slowdown in relaxation as the system enters the non-Markovian regime. This observation evidences the non-negligible influence of non-Markovian effects on the dynamics.

Further insights are revealed by analyzing the eigenenergy spectrum in Fig.~\ref{fig:eigen}. Especially, at low $\Gamma$, both HEOM and BMME exhibit consistent eigenenergy distributions. However, as $\Gamma$ approaches the non-Markovian regime, a characteristic shift towards zero emerges in the HEOM eigenenergies. This spectral signature directly reflects the non-perturbative slowdown in relaxation caused by non-Markovian effects beyond the secular approximation.

\begin{figure}[]
	\centering
    \includegraphics[width = 1\columnwidth]{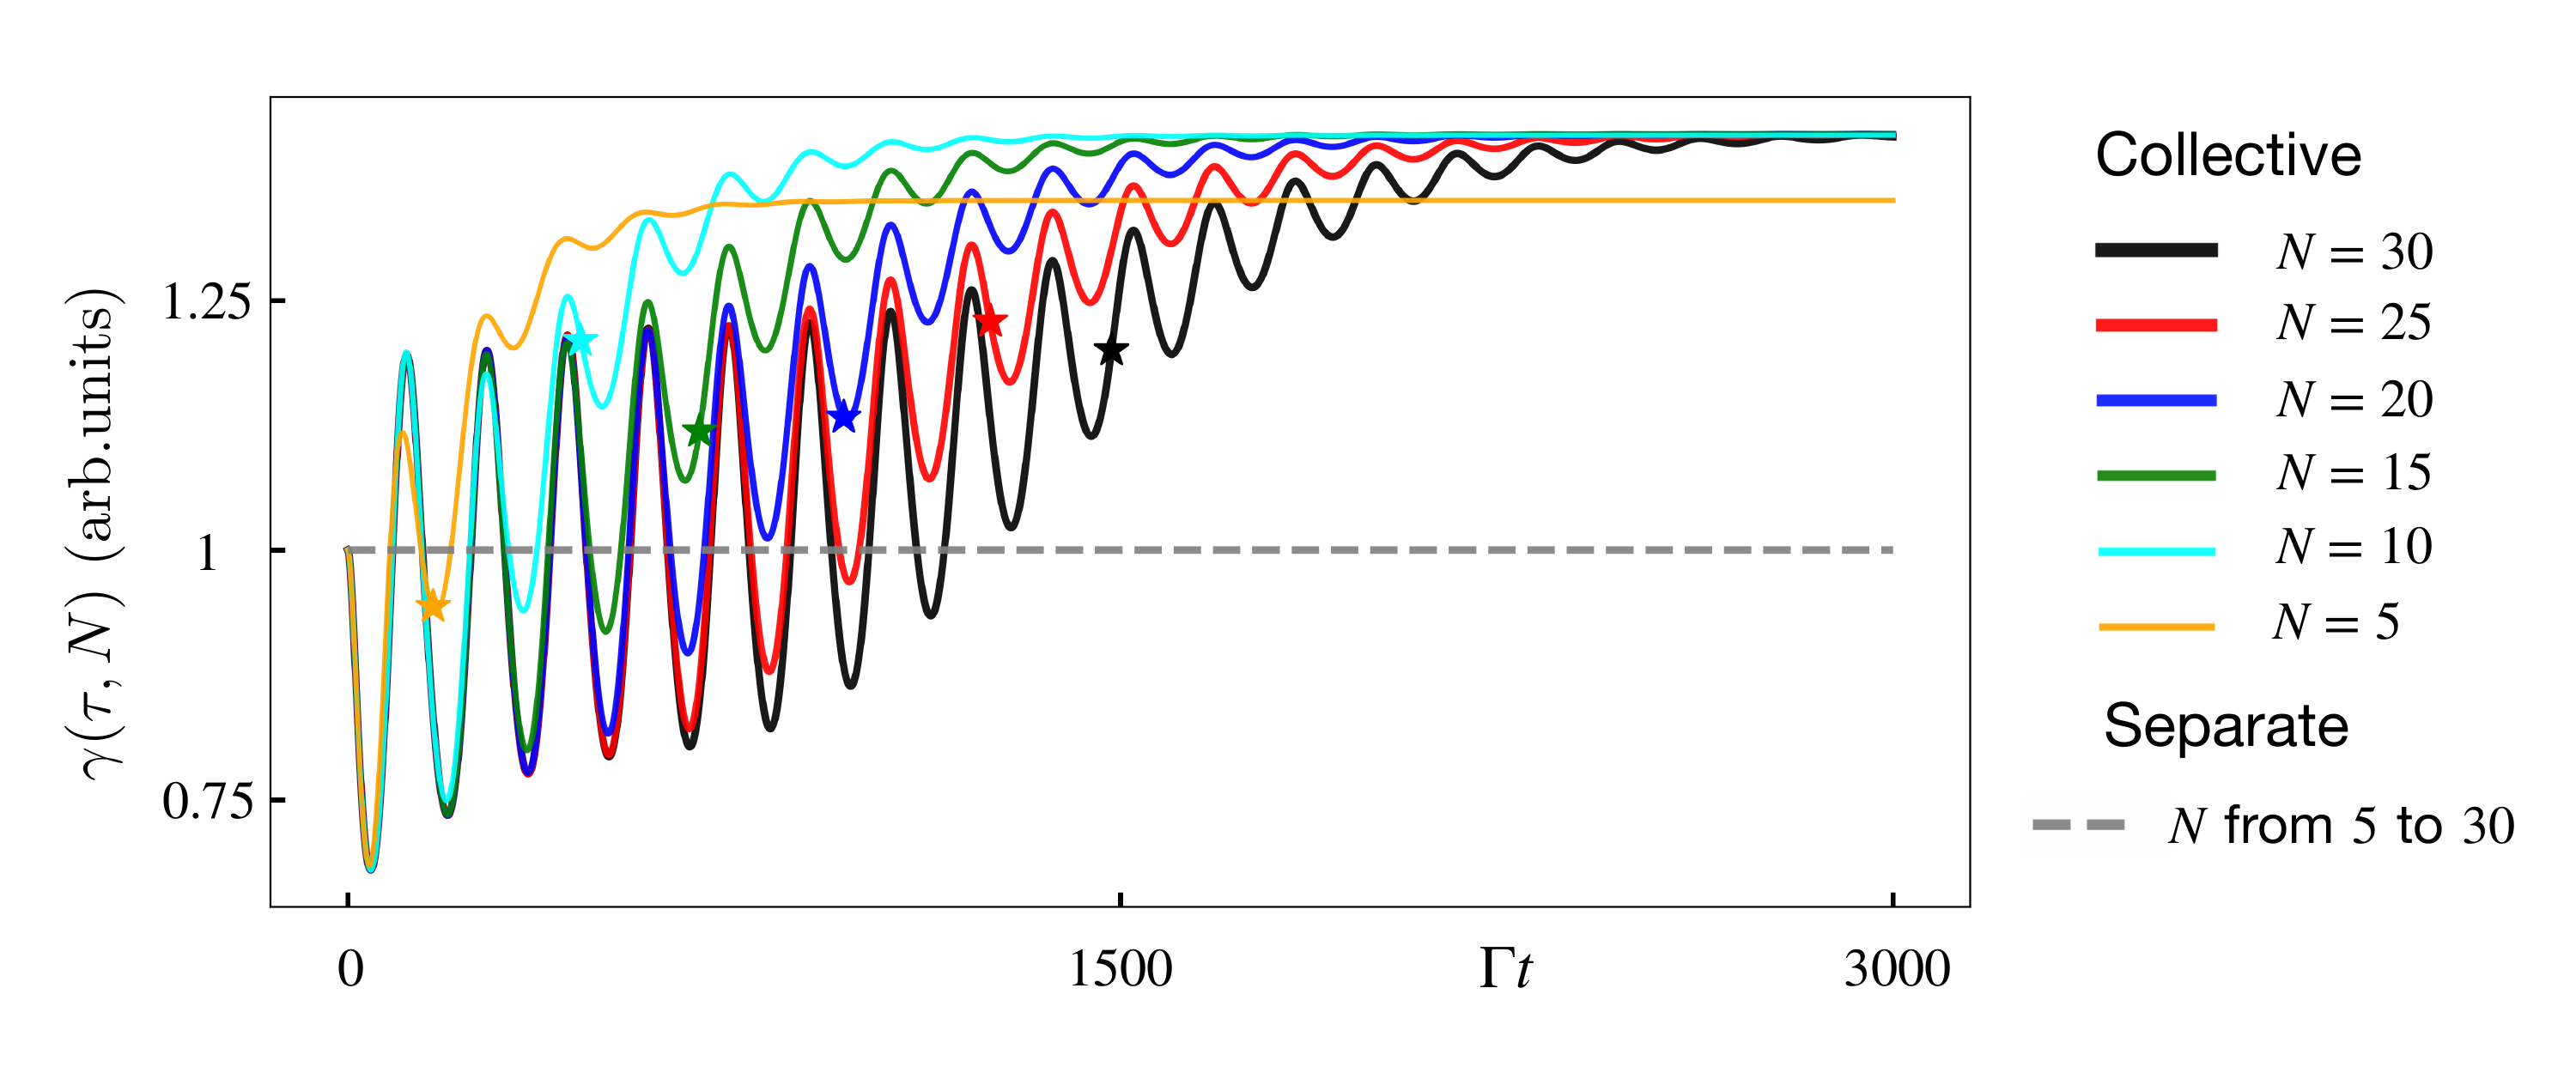}
	\caption{Evolution of the scaled emission rate, $\gamma(t,N)$, over time $t$ for system sizes $N=5$ to $30$, under both collective (solid curves) and separated (dashed curves) coupling conditions at a fixed coupling strength $\Gamma=0.5\Omega$. The star symbols indicate the scaled emission rate at a given relaxation time $\tau$.}
	\label{fig:superadient}
\end{figure}
\section{Scaled emission rate and inter-site coherence}
Quantum coherence arises in many-body systems like optical lattices or dense emitter ensembles. To observe and quantify this phenomenon, we analyze the scaled emission rate, which incorporates both single-site and collective emission contributions:
\begin{equation}
\begin{aligned}
\gamma(t,N)\approx\sum_{n=1}^{N}\Big[\langle d_{n}^{\dagger}d_{n}\rangle(t)+\sum_{m\neq n}\langle d_{m}^{\dagger}d_{n}\rangle(t)\Big].
\label{eq:scaled_rate}
\end{aligned}
\end{equation}
It considers the time dependence, $t$, and the number of sites, $N$. The first term represents single-site emission, while the second captures the collective effect arising from correlations between different sites.

Crucially, the system's bath coupling configuration impacts the observed coherence. For models with separated coupling to different baths (Fig.~\ref{fig:superadient}), $\gamma(t,N)$ remains near unity. This signifies the absence of significant quantum correlations, as the separated coupling configuration cannot induce collective coherence.

Conversely, models with collective coupling to a common bath exhibit pronounced coherence. As shown in Fig.~\ref{fig:superadient}, $\gamma(t,N)$ exceeds unity due to the non-negligible collective term representing quantum correlations.

Since $\gamma(t,N)$ oscillates with $t$, we average it over time for each $N$ to assess the coherence contribution to non-Markovian relaxation. This average scaled rate, presented in Eq.~(9) of the main text, underscores the presence and significance of quantum correlations.

\begin{figure}[]
	\centering
    \includegraphics[width = 1.0\columnwidth]{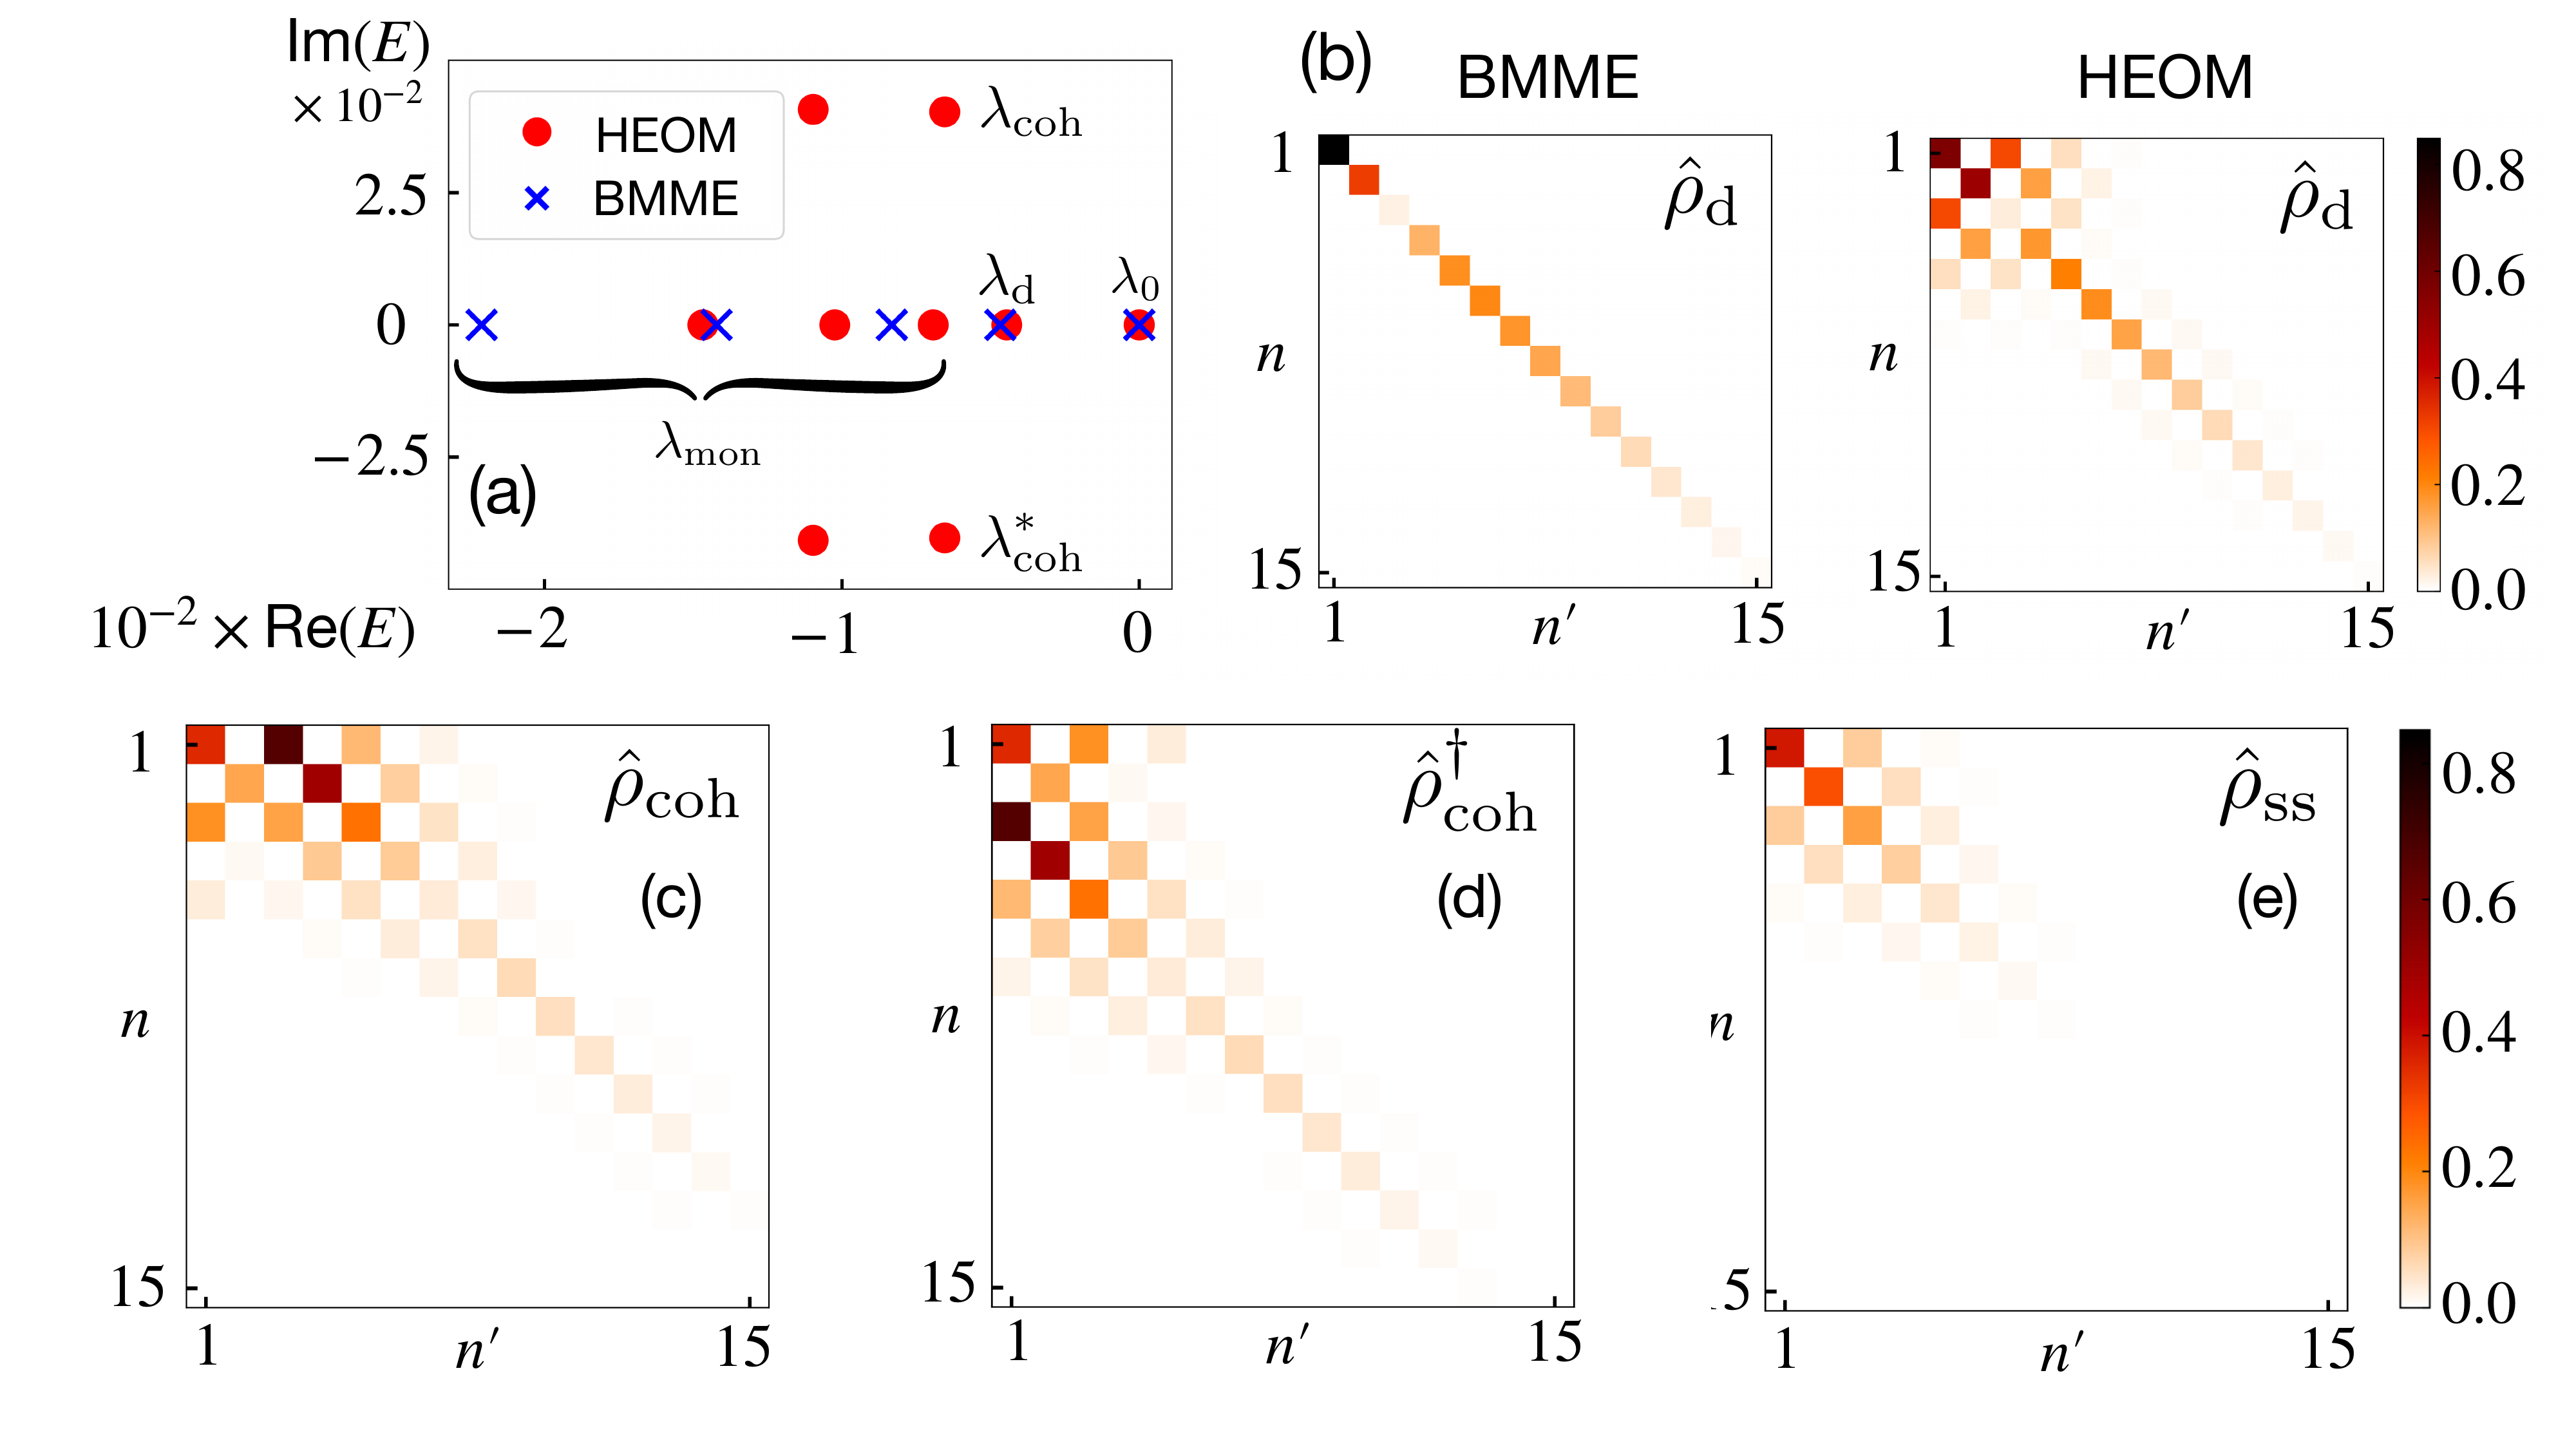}
	\caption{Eigenvalue spectrum and density matrix analysis of the non-Markovian skin effect. (a) Comparison of eigenspectra obtained from BMME (blue crosses) and HEOM (red circles) approaches. Key eigenvalues $\lambda_0$, $\lambda_d$, $\lambda_{\text{coh}\pm}$, and $\lambda_{\text{mon}}$ correspond to steady-state, dominant skin mode, secondary skin modes, and monotonic decay modes, respectively. (b) Color plots depicting absolute values of the reduced density matrix $\hat{\rho}_{\text{d}}$ for $N=15$, comparing BMME (left) and HEOM (right) results. (c-e) Color plots depicting absolute values of the reduced density matrix elements for key eigenmodes in the HEOM approach: (c) $\hat{\rho}_{\text{coh}}$, (d) $\hat{\rho}_{\text{coh}+}^{\dagger}$, and (e) steady-state $\hat{\rho}_{\text{ss}}$. The color scale indicates the magnitude of the matrix elements, highlighting the emergence of cross-site coherence in the non-Markovian regime.}
	\label{eigenspectrum}
\end{figure}

\section{Non-Markovian eigenvalue spectrum}

The non-Markovian skin effect exhibits unique characteristics beyond those observed in  Markovian systems. As discussed in the main text, while the primary skin mode dominates the relaxation process, the secondary skin modes $\hat{\pmb{\rho}}_{\text{coh}}^{(\dagger)}$ with complex eigenvalues $\lambda_{\text{coh}}^{(*)}$ play a crucial role in inducing the oscillatory behavior during relaxation.

Figure.~\ref{eigenspectrum}(a) compares the eigenvalue spectra obtained from HEOM and BMME approaches. In the Markovian limit (BMME), the secondary skin modes induced by the non-Markovian effects and virtual processes are absent. Moreover, the virtual processes facilitated by the counter-rotating terms in the strong coupling regime induce cross-site coherence, leading to distinctive oscillatory behavior in the non-Markovian skin effect. This cross-site coherence within the relaxation dynamics is contributed to by both the primary skin mode and secondary skin modes, as illustrated in Figures \ref{eigenspectrum}(b), (c), and (d). Notably, the pair of secondary skin modes $\hat{\pmb{\rho}}_{\text{coh}}^{(\dagger)}$ with complex eigenvalues $\lambda_{\text{coh}}^{(*)}$ are conjugates of each other. Furthermore, this coherence persists even in the long-time limit, as evidenced by thecross-site coherence in the steady-state eigenmode [Fig.~\ref{eigenspectrum}(e)]. Such cross-site coherence cannot be captured by BMME in the Markovian limit, even when $\Gamma$ is in the strong coupling regime (Fig.~\ref{eigenspectrum}(b)).

\begin{figure}[]
	\centering
    \includegraphics[width = 1.0\columnwidth]{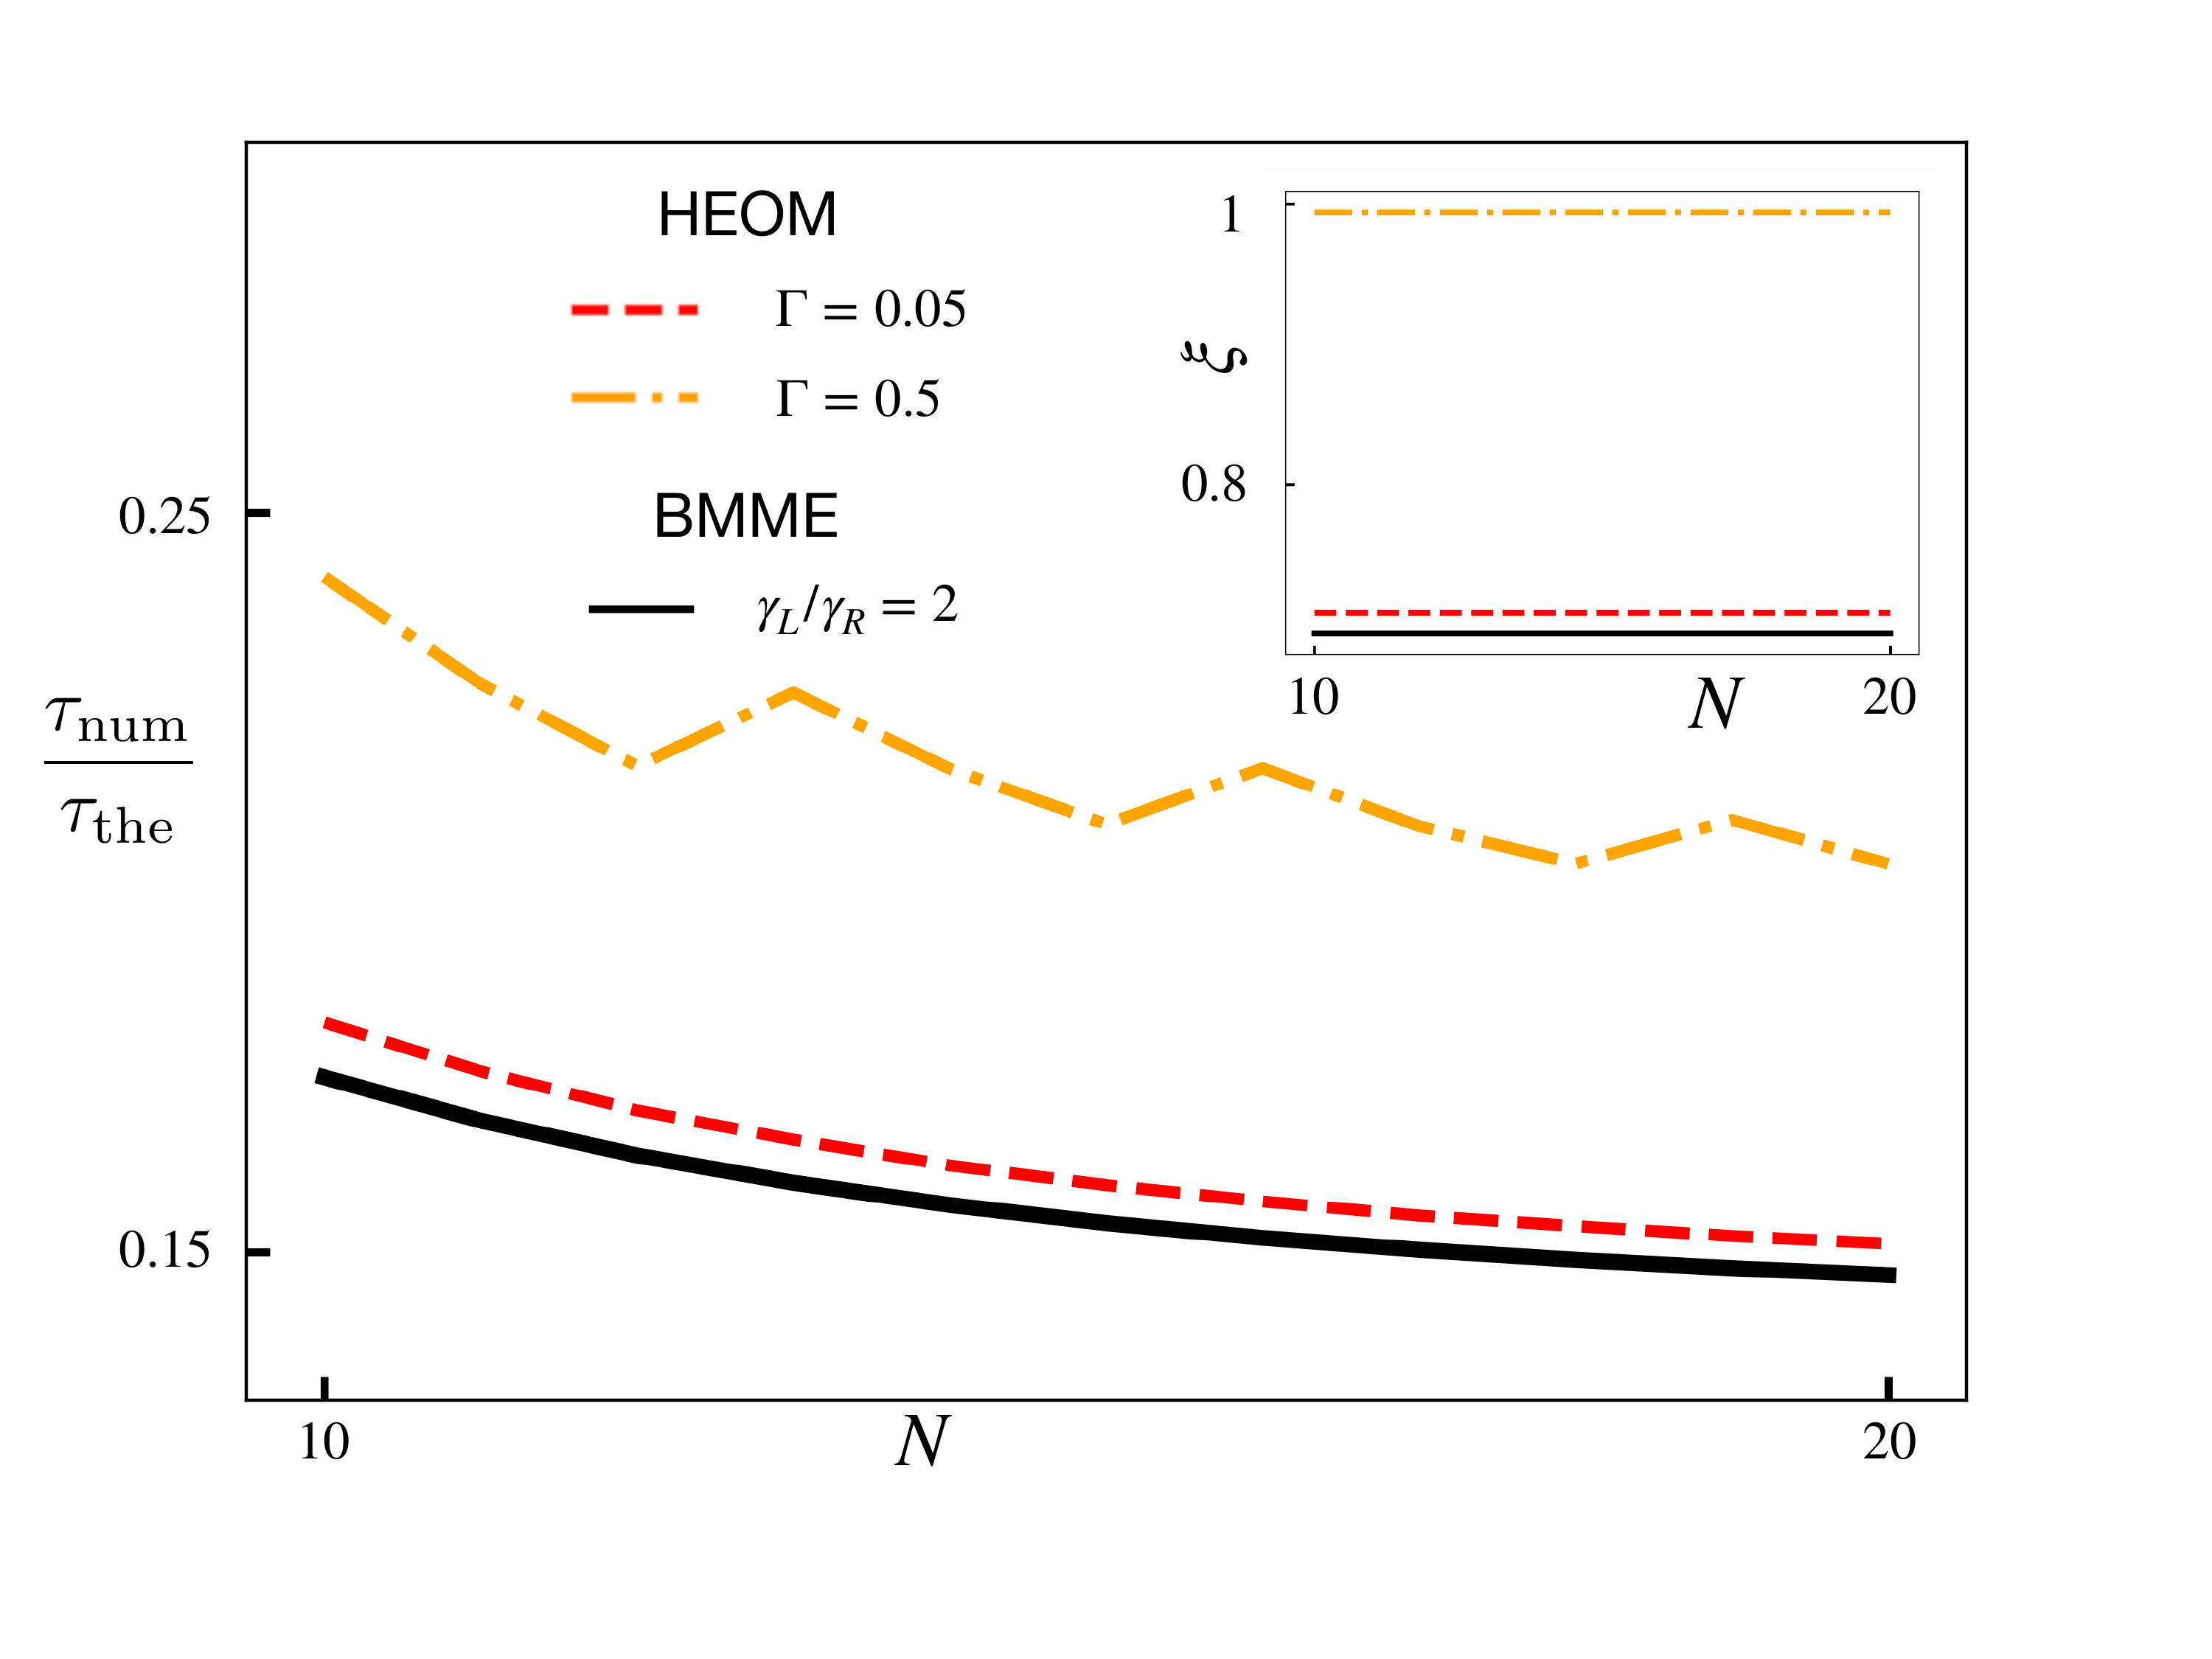}
	\caption{Comparison of numerical and analytical relaxation times across different system sizes and coupling strengths. Main plot: Ratio of numerical ($\tau_\text{num}$) to analytical ($\tau_\text{the}$) relaxation times for system sizes $N=10$ to $20$. Results are shown for HEOM with weak ($\Gamma=0.05$, red dashed line) and strong ($\Gamma=0.5$, orange dash-dotted line) coupling, and BMME ($\gamma_L/\gamma_R=2$, black solid line). Inset: Localization length $\xi$ of the dominant eigenmode $\rho_\text{d}$ as a function of system size $N$, comparing Markovian (BMME) and non-Markovian (HEOM) regimes for different coupling strengths. }
	\label{localization_length}
\end{figure}

With the information of eigenvalue spectrum, we can evaluate the relationship between the relaxation time $\tau$ and system size $N$, incorporating the dominant eigenvalue $\lambda_{\text{d}}$ and localization length $\xi_{\text{H}}$. The localization length $\xi_{\text{H}}$ can be determined by using any eigenmode contributing to the system dynamics (Fig.~\ref{eigenspectrum}). In the Markovian regime, $\xi$ is related to the ratio of leftward ($\gamma_L$) and rightward ($\gamma_R$) hopping strengths by $\xi \sim |\ln(\gamma_L/\gamma_R)|^{-1}$. As the effective hopping strength in HEOM is related to $\Gamma$, the trend of $\xi_{\text{H}}$ with respect to $N$ remains consistent for any $\rho_i$ at fixed $\Gamma$.

To extract $\xi_{\text{H}}$, we numerically fit the spatial distribution of $\rho_i$ as a function of site $n$ using $f(n,\xi_{\text{H}}) \sim a \exp(-n/\xi_{\text{H}})$. While the steady-state eigenmode offers easier fitting due to less spatial oscillation, we use $\rho_{\text{d}}$ to evaluate $\xi_{\text{H}}$ for consistency with our relaxation time formula [Eq.~(6) in the main text].

Fig.~\ref{localization_length} demonstrates that using $\rho_{\text{d}}$ to obtain $\xi_{\text{H}}$ aligns well with Eq.~(6). By substituting $\lambda_{\text{d}}$ and $\xi_{\text{H}}$ obtained from $\rho_{\text{d}}$ into Eq.~(6), we derive the analytical relaxation time $\tau_{\text{the}}$ as a function of $N$
\begin{equation}\label{LSE}
\tau_\text{the}=\frac{1}{\lambda_{\text{d}}} + \frac{N}{\lambda_{\text{d}} \xi_{\text{H}}}.
\end{equation}
We compare this with the numerical relaxation time $\tau_{\text{num}}$ extracted from HEOM simulations. For relatively weak coupling ($\Gamma=0.05\Omega$), the ratio $\tau_{\text{num}}/\tau_{\text{the}}$ obtained by HEOM closely aligns with the BMME results, validating Eq.~(6) in the non-Markovian regime. In the strong coupling regime ($\Gamma=0.5\Omega$), while the ratio remains close, it exhibits additional oscillatory behavior, consistent with our main results showing $\tau$ oscillations due to secondary skin mode effects in the non-Markovian regime. To elucidate the mechanism behind these oscillations, we re-examine the non-Markovian effects from a microscopic perspective. 

Firstly, we observe a strong correlation between the oscillatory trend of $\tau$ and the scaled rate for particle transport, $\bar{\gamma}(\tau,N)$, revealing a coherence signature within the system. The oscillations in $\bar{\gamma}(\tau,N)$ with respect to system size, $N$, originate from the significant oscillations in the time-dependent rate, $\gamma(t,N)=\sum_{n=1}^{N}[\langle d_{n}^{\dagger}d_{n}\rangle(t)+\sum_{m\neq n}\langle d_{m}^{\dagger}d_{n}\rangle(t)]$ [illustrated for $N=21$ to $23$ in Fig.~\ref{21_23}(a)]. The secondary skin mode, characterized by the eigenvalues with an imaginary component ($\text{Im}[\lambda_{\text{coh}}^{(\dagger)}]$), induces oscillatory behavior in the system's coherence, $\langle d_m^\dagger d_n \rangle(t)$ [Fig.~\ref{21_23}(b)]. As $\bar{\gamma}(\tau,N)$ is the time integral of $\gamma(t,N)$ up to $\tau$, the oscillations in $\langle d_m^\dagger d_n \rangle(t)$ directly translate to oscillations in $\bar{\gamma}(\tau,N)$ with varying $N$. While the oscillation frequency of $\gamma(t,N)$ remains constant due to the consistent $\text{Im}[\lambda_{\text{coh}}^{(\dagger)}]$, $\tau$ varies with $N$, particularly as $\lambda_d$ approaches zero with increasing $N$. This results in markedly different $\gamma(\tau,N)$ values at the upper limit $\tau$, despite the constant frequency. Thus, the oscillations of $\bar{\gamma}(\tau,N)$ with $N$ are modulated by both primary and secondary skin modes, reflecting the interplay between system size and relaxation dynamics.

Secondly, as detailed in the revised manuscript, the counter-rotating terms in the interaction Hamiltonian play a pivotal role. Specifically, quantum coherence emerges only for "cross-site" pairs, such as $(n, m) = (1, 3)$, $(2, 4)$, and even $(3, 5)$, $(4, 6)$, with no coherence between adjacent sites. This is illustrated in Fig. 4(c) of the main text, where only cross-site $\langle d_{n}^{\dagger}d_{m}\rangle(t)$ terms contribute significantly to $\gamma(t, N)$.

An intuitive picture of this effective cross-site coupling, $\langle d_{n}^{\dagger}d_{m}\rangle(t)$, can be conceptualized using a three-site model: A particle transitioning from the third site to the second site, via the conventional transition operator $d_{n}^{\dagger}d_{n+1} a_k^{\dagger}$, generates a boson. This boson can subsequently undergo a virtual process (higher-order transition) facilitated by the counter-rotating term $d_{n}^{\dagger}d_{n+1} a_k$, enabling the particle to further transit to the first site. This composite transition process generates the cross-site $\langle d_{n}^{\dagger}d_{m}\rangle(t)$ terms, thereby creating the cross-site quantum correlations. Consequently, while no such coherence exists for a two-site system ($N=2$), it emerges when $N=3$ (i.e., the coherence between the first and third sites), contributing to $\bar{\gamma}(\tau,N)$ and resulting in a sudden increase in its value. This pattern extends to larger system sizes, with similar sudden increases at specific intervals due to the emergence of cross-site coherence, leading to the periodic behavior of $\bar{\gamma}(\tau,N)$.

\begin{figure}[]
	\centering
    \includegraphics[width = 1.\columnwidth]{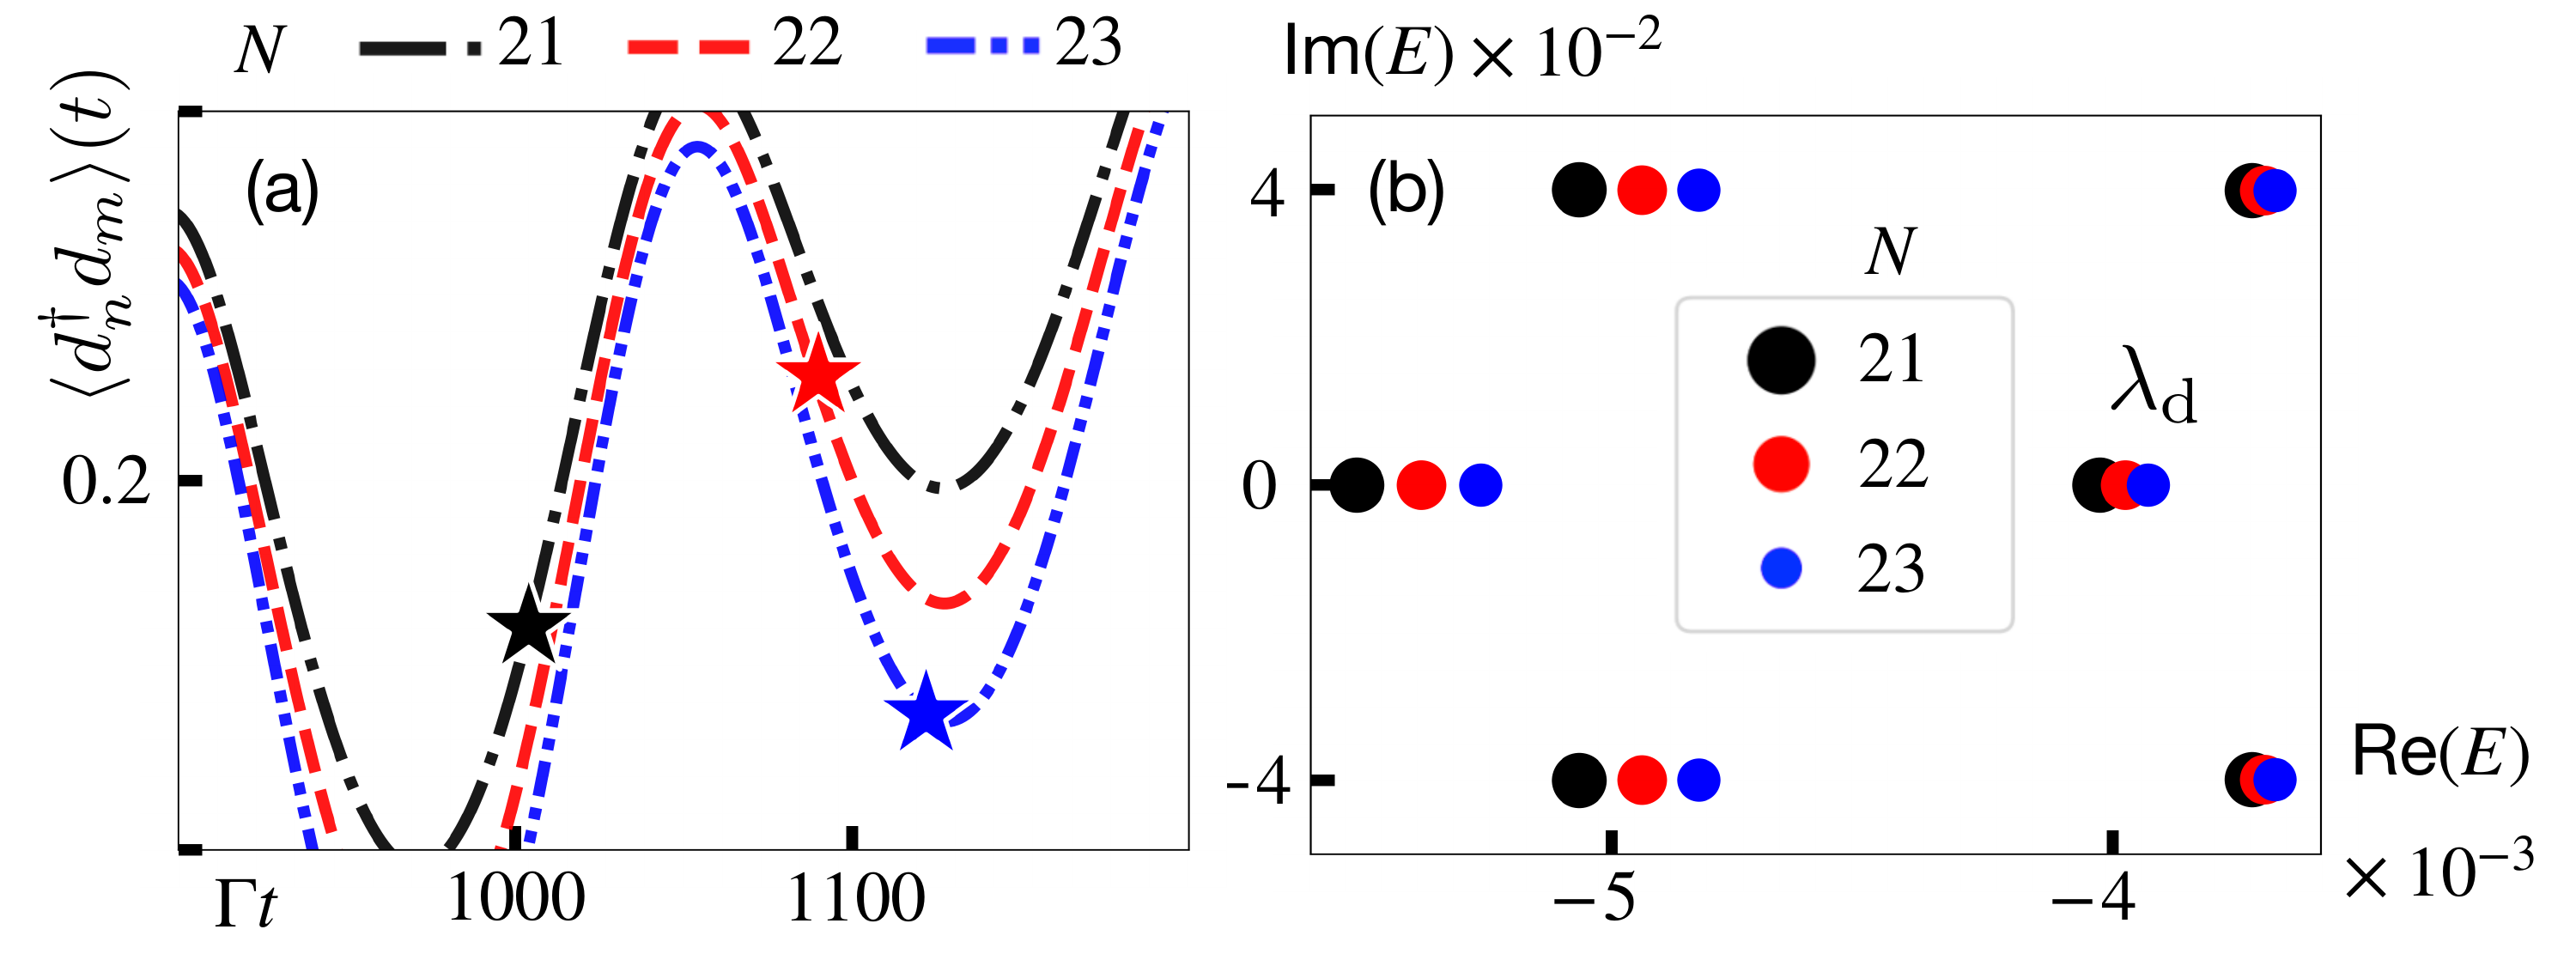}
	\caption{The time evolutions of the cross-site coherence $\langle d_m^\dagger d_n \rangle(t)$ exhibit significant oscillations (a), primarily driven by the secondary skin mode due to its imaginary eigenvalue component (b). This oscillatory behavior directly influences the relaxation time $\bar{\gamma}(\tau,N)$, obtained by integrating $\gamma(t,N)$ (which includes $\langle d_m^\dagger d_n \rangle(t)$) up to $\tau$ for each system size $N$ and then averaging over $\tau$. As illustrated for $N = 21$, 22, and 23, the relaxation time points (marked by stars) for $\langle d_m^\dagger d_n \rangle(t)$ coincide with a trough, a peak, and another trough, respectively, following the oscillatory trend observed in $\bar{\gamma}(\tau,N)$.}
	\label{21_23}
\end{figure}

In conclusion, the oscillatory behavior of $\bar{\gamma}(\tau,N)$ arises from the interplay of two key factors: the emergence of cross-site coherence due to virtual processes facilitated by counter-rotating terms, and the complex eigenenergies of the secondary skin mode, which induce oscillations in the system's coherences. The former provides a physical origin for the observed periodicity, while the latter serves as the underlying mathematical mechanism. These mechanisms are inherently non-Markovian and absent in the Markovian limit, highlighting the unique characteristics of non-Markovian open quantum systems.

%\bibliography{ref}

\end{document}
